# Supplementary material for: Matrix Quantile Factor Model
Source: arXiv:2208.08693 source file (2024-08-20)
Supplement: Supplementary file 1 [file Online_Appendix_for____Matrix_Quantile_Factor_Model___5-26.pdf]

# Online Appendix for “Matrix Quantile Factor Model”

Xin-Bing Kong, Yong-Xin Liu, Long Yu and Peng Zhao

May 26, 2023

## A Preliminaries

This section introduces some definitions used in the following proof.

Let

$$r_i = \begin{pmatrix} r_{1i} \\ r_{2i} \\ \vdots \\ r_{k_1 i} \end{pmatrix}_{k_1 \times 1}, \mathbf{F}_t = \begin{pmatrix} f_{t11} & \cdots & f_{t1k_2} \\ \vdots & \ddots & \vdots \\ f_{tk_1 1} & \cdots & f_{tk_1 k_2} \end{pmatrix}_{k_1 \times k_2}, c_j = \begin{pmatrix} c_{1j} \\ c_{2j} \\ \vdots \\ c_{k_2 j} \end{pmatrix}_{k_2 \times 1}$$

and the quantile-dependent idiosyncratic error  $\varepsilon_{ijt}$  satisfies the quantile restrictions,

$$P[\varepsilon_{ijt}(\tau) \leq 0 | F_t(\tau)] = \tau, \quad \text{a.s.}$$

Let

$$\mathbf{R} = \begin{pmatrix} r'_1 \\ r'_2 \\ \vdots \\ r'_{p_1} \end{pmatrix}_{p_1 \times k_1}, \mathbf{C} = \begin{pmatrix} c'_1 \\ c'_2 \\ \vdots \\ c'_{p_2} \end{pmatrix}_{p_2 \times k_2},$$

$M = p_1 k_1 + T k_1 k_2 + p_2 k_2$ , and  $\theta_0 = (r'_{01}, \dots, r'_{0p_1}, \mathbf{F}_{01}, \dots, \mathbf{F}_{0T}, c'_{01}, \dots, c'_{0p_2})'$  denoting the vector of true parameters. For any  $\theta_a, \theta_b \in \Theta^{k_1 k_2}$ , define the semimetric  $d$  by

$$d(\theta_a, \theta_b) = \sqrt{\sum_{i=1}^{p_1} \sum_{t=1}^T \sum_{j=1}^{p_2} \frac{(r'_{ai} \mathbf{F}_{at} c'_{aj} - r'_{bi} \mathbf{F}_{bt} c'_{bj})^2}{p_1 p_2 T}} = \sqrt{\sum_{t=1}^T \frac{\|\mathbf{R}_a \mathbf{F}_{at} \mathbf{C}'_a - \mathbf{R}_b \mathbf{F}_{bt} \mathbf{C}'_b\|^2}{p_1 p_2 T}},$$

and let  $w_{ijt}(r_i, \mathbf{F}_t, c_j) = \rho_\tau(X_{ijt} - r'_i \mathbf{F}_t c_j) - \rho_\tau(X_{ijt} - r'_{0i} \mathbf{F}_{0t} c_{0j})$ ,

$$\mathbb{M}_{p_1 p_2 T}^*(\theta) = \sum_{i=1}^{p_1} \sum_{t=1}^T \sum_{j=1}^{p_2} \frac{w_{ijt}(r_i, \mathbf{F}_t, c_j)}{p_1 p_2 T}, \quad \bar{\mathbb{M}}_{p_1 p_2 T}^*(\theta) = \sum_{i=1}^{p_1} \sum_{t=1}^T \sum_{j=1}^{p_2} \frac{\mathbb{E}[w_{ijt}(r_i, \mathbf{F}_t, c_j)]}{p_1 p_2 T}.$$

## B Proof of Theorem 3.2

This section provides the detailed technical proof of Theorem 3.2.

### B.1 Definitions and Notations

For a matrix  $A$  with real eigenvalues,  $\rho_j(A)$  denotes the  $j$ th largest eigenvalue. For a square matrix  $A$  whose  $j$ th diagonal element is denoted as  $A_{jj}$ . Following van der Vaart and Wellner (1996), the symbol  $\lesssim$  means “left side bounded by a positive constant times the right side” (the symbol  $\gtrsim$  is defined similarly).  $D(\cdot, g, \mathcal{G})$  and  $C(\cdot, g, \mathcal{G})$  denotes the packing number and covering number of space  $\mathcal{G}$  endowed with semimetric  $g$ .

Throughout the Appendix,  $K_1, K_2, \dots$  denote some positive constants that do not depend on  $p_1, p_2, T$ . For any random variable  $Y$ , define the Orlicz norm  $\|Y\|_\psi$  as

$$\|Y\|_\psi = \inf\{C > 0 : \mathbb{E}_\psi(|Y|/C) \leq 1\},$$

where  $\psi$  is a non-decreasing, convex function with  $\psi(0) = 0$ . In particular, when  $\psi(x) = e^{x^2} - 1$ , the norm is written as  $\|Y\|_{\psi_2}$ . We use  $\|\cdot\|_S$  to denote the spectral norm, and  $C(\cdot, g, \mathcal{G})$  to denote the covering number of space  $\mathcal{G}$  endowed with semimetric  $g$ . Moreover, define

$$\mathbb{W}_{p_1 p_2 T}(\theta) = \mathbb{M}_{p_1 p_2 T}^*(\theta) - \bar{\mathbb{M}}_{p_1 p_2 T}^*(\theta) = \frac{1}{p_1 p_2 T} \sum_{i=1}^{p_1} \sum_{j=1}^{p_2} \sum_{t=1}^T (\omega_{ijt}(r_i, \mathbf{F}_t, c_j) - \mathbb{E}[\omega_{ijt}(r_i, \mathbf{F}_t, c_j)]),$$

where  $\omega_{ijt}(r_i, \mathbf{F}_t, c_j) = \rho_\tau(X_{ijt} - r'_i \mathbf{F}_t c_j) - \rho_\tau(X_{ijt} - r'_{0i} \mathbf{F}_{0t} c_{0j})$ .

### B.2 Three Preliminary Lemmas

This subsection presents three preliminary lemmas to prove the Theorem 3.2.

**Lemma B.1.** *Under Assumption 1, it holds that  $d(\hat{\theta}, \theta_0) = o_p(1)$  as  $p_1, p_2, T \rightarrow \infty$ .*

*Proof.* First, for any  $r_i \in \mathcal{A}, \mathbf{F}_t \in \mathcal{F}, c_j \in \mathcal{B}$ , expanding  $\mathbb{E}[\rho_\tau(X_{ijt} - r'_i \mathbf{F}_t c_j) - \rho_\tau(X_{ijt} - r'_{0i} \mathbf{F}_{0t} c_{0j})]$  around  $c_{0,ijt} = r'_{0i} \mathbf{F}_{0t} c_{0j}$ , we have

$$\mathbb{E}[\rho_\tau(X_{ijt} - r'_i \mathbf{F}_t c_j) - \rho_\tau(X_{ijt} - r'_{0i} \mathbf{F}_{0t} c_{0j})] = 0.5 f_{ijt}(\tilde{c}_{ijt}) \cdot (r'_i \mathbf{F}_t c_j - r'_{0i} \mathbf{F}_{0t} c_{0j})^2,$$

where  $\tilde{c}_{ijt}$  is between  $r'_i \mathbf{F}_t c_j$  and  $c_{0,ijt}$ . It then follows from Assumption 1-2 that for all  $r_i \in \mathcal{A}, \mathbf{F}_t \in \mathcal{F}, c_j \in \mathcal{B}$ ,

$$\mathbb{E}[\rho_\tau(X_{ijt} - r'_i \mathbf{F}_t c_j) - \rho_\tau(X_{ijt} - r'_{0i} \mathbf{F}_{0t} c_{0j})] \gtrsim (r'_i \mathbf{F}_t c_j - r'_{0i} \mathbf{F}_{0t} c_{0j})^2$$

since  $|r'_i \mathbf{F}_t c_j|$  and  $|r'_{0i} \mathbf{F}_{0t} c_{0j}|$  are both bounded. Therefore, for any  $\theta \in \Theta^{k_1 k_2}$ , we have

$$\bar{\mathbb{M}}_{p_1 p_2 T}^*(\theta) \gtrsim d^2(\theta, \theta_0). \quad (1)$$

Second, by the definition of  $\hat{\theta}$ , we have  $\mathbb{M}_{p_1 p_2 T}^*(\hat{\theta}) = \mathbb{M}_{p_1 p_2 T}(\hat{\theta}) - \mathbb{M}_{p_1 p_2 T}(\theta_0) \leq 0$ , or equivalently  $\mathbb{W}_{p_1 p_2 T}(\hat{\theta}) + \bar{\mathbb{M}}_{p_1 p_2 T}^*(\hat{\theta}) \leq 0$ . It then follows from (1) that

$$0 \leq d^2(\hat{\theta}, \theta_0) \lesssim \bar{\mathbb{M}}_{p_1 p_2 T}^*(\hat{\theta}) \leq \sup_{\theta \in \Theta^{k_1 k_2}} |\mathbb{W}_{p_1 p_2 T}(\theta)|.$$

Thus, it remains to show that

$$\sup_{\theta \in \Theta^{k_1 k_2}} |\mathbb{W}_{p_1 p_2 T}(\theta)| = o_p(1). \quad (2)$$

Choose  $K_1, K_2, K_3$  large enough such that  $\|r_{0i}\|, \|r_i\| \leq K_1$  for all  $i$ ,  $\|c_{0j}\|, \|c_j\| \leq K_2$  for all  $j$ ,  $\|\mathbf{F}_{0t}\|, \|\mathbf{F}_t\| \leq K_3$  for all  $t$ , for any  $\theta \in \Theta^{k_1 k_2}$ . Let  $B_{k_1}(K_1)$  be a Euclidean ball in  $\mathbb{R}^{k_1}$  with radius  $K_1$ . For any  $\epsilon > 0$ , let  $r_{(1)}, \dots, r_{(J_1)}$  be a maximal set of points in  $B_{k_1}(K_1)$  such that  $\|r_{(j)} - r_{(h)}\| > \epsilon/K_1$  for any  $j \neq h$  where “maximal” signifies that no point can be added without violating the validity of the inequality. Similarly, let  $B_{k_2}(K_2)$  be a Euclidean ball in  $\mathbb{R}^{k_2}$  with radius  $K_2$ . Let  $c_{(1)}, \dots, c_{(J_2)}$  be a maximal set of points in  $B_{k_2}(K_2)$  such that  $\|c_{(j)} - c_{(h)}\| > \epsilon/K_2$  for any  $j \neq h$ . Let  $B_{k_1, k_2}(K_3)$  be a Euclidean ball in  $\mathbb{R}^{k_1 \times k_2}$  with radius  $K_3$ . Let  $\mathbf{F}_{(1)}, \dots, \mathbf{F}_{(J_3)}$  be a maximal set of points in  $B_{k_1, k_2}(K_3)$  such that  $\|\mathbf{F}_{(j)} - \mathbf{F}_{(h)}\| > \epsilon/K_3$  for any  $j \neq h$ . It is well

known that  $J_1, J_2$  and  $J_3$ , the packing numbers of  $B_{k_1}(K_1)$ ,  $B_{k_2}(K_2)$  and  $B_{k_1, k_2}(K_3)$  are equal to  $K_4(K_1/\epsilon)^{k_1}$ ,  $K_5(K_2/\epsilon)^{k_2}$  and  $K_6(K_3/\epsilon)^{k_1 k_2}$ , respectively.

For any  $\theta \in \Theta^{k_1 k_2}$ , define  $\theta^* = (r_1^{*'}, \dots, r_{p_1}^{*'}, \mathbf{F}_1^{*'}, \dots, \mathbf{F}_T^{*'}, c_1^{*'}, \dots, c_{p_2}^{*'})'$ , where  $r_i^* = \{r_{(j)} : j \leq J_1, \|r_{(j)} - r_i\| \leq \epsilon/K_1\}$ ,  $c_j^* = \{c_{(j)} : j \leq J_2, \|c_{(j)} - c_j\| \leq \epsilon/K_2\}$  and  $\mathbf{F}_t^* = \{\mathbf{F}_{(j)} : j \leq J_3, \|\mathbf{F}_{(j)} - \mathbf{F}_t\| \leq \epsilon/K_3\}$ . Thus, we can write

$$\mathbb{W}_{p_1 p_2 T}(\theta) = \mathbb{W}_{p_1 p_2 T}(\theta^*) + \mathbb{W}_{p_1 p_2 T}(\theta) - \mathbb{W}_{p_1 p_2 T}(\theta^*).$$

Note that

$$\begin{aligned} & |\rho_\tau(X_{ijt} - r_i' \mathbf{F}_t c_j) - \rho_\tau(X_{ijt} - r_i^{*'} \mathbf{F}_t^* c_j^*)| \\ & \leq 2|r_i' \mathbf{F}_t c_j - r_i^{*'} \mathbf{F}_t^* c_j^*| \\ & \leq 2(\|r_i'\| \|\mathbf{F}_t\| \|c_j - c_j^*\| + \|r_i'\| \|\mathbf{F}_t - \mathbf{F}_t^*\| \|c_j^*\| + \|r_i' - r_i^{*'}\| \|\mathbf{F}_t^*\| \|c_j^*\|) \\ & \leq 6\epsilon \end{aligned}$$

Thus,

$$\sup_{\theta \in \Theta^{k_1 k_2}} |\mathbb{W}_{p_1 p_2 T}(\theta) - \mathbb{W}_{p_1 p_2 T}(\theta^*)| \leq 6\epsilon. \quad (3)$$

Also, note that

$$|\omega_{ijt}(r_i^*, \mathbf{F}_t^*, c_j^*)| = |\rho_\tau(X_{ijt} - r_i^{*'} \mathbf{F}_t^* c_j^*) - \rho_\tau(X_{ijt} - r_{0i}' \mathbf{F}_{0t} c_{0j})| \leq 2|r_i^{*'} \mathbf{F}_t^* c_j^* - r_{0i}' \mathbf{F}_{0t} c_{0j}|.$$

Then,  $\mathbb{W}_{p_1 p_2 T}(\theta^*) = \frac{1}{p_1 p_2 T} \sum_{i=1}^{p_1} \sum_{t=1}^T \sum_{j=1}^{p_2} (\omega_{ijt}(r_i^*, \mathbf{F}_t^*, c_j^*) - E[\omega_{ijt}(r_i^*, \mathbf{F}_t^*, c_j^*)]) = \overline{W} - E(\overline{W})$ , where  $\overline{W} = \frac{1}{p_1 p_2 T} \sum_{i=1}^{p_1} \sum_{t=1}^T \sum_{j=1}^{p_2} W_{ijt}$  with  $W_{ijt} = \omega_{ijt}(r_i^*, \mathbf{F}_t^*, c_j^*)$ . By Hoeffding's inequality

$$\begin{aligned} & P(|\sqrt{p_1 p_2 T} \mathbb{W}_{p_1 p_2 T}(\theta^*)| > c) \\ & = P(|\overline{W} - E(\overline{W})| > \frac{c}{\sqrt{p_1 p_2 T}}) \\ & \leq 2 \exp \left( - \frac{2(p_1 p_2 T)^2 (\frac{c}{\sqrt{p_1 p_2 T}})^2}{4 \sum_{i=1}^{p_1} \sum_{t=1}^T \sum_{j=1}^{p_2} (r_i^{*'} \mathbf{F}_t^* c_j^* - r_{0i}' \mathbf{F}_{0t} c_{0j})^2} \right) \\ & = 2 \exp \left( - \frac{c^2}{2 \sum_{i=1}^{p_1} \sum_{t=1}^T \sum_{j=1}^{p_2} (r_i^{*'} \mathbf{F}_t^* c_j^* - r_{0i}' \mathbf{F}_{0t} c_{0j})^2 / p_1 p_2 T} \right) \\ & = 2 \exp \left( - \frac{c^2}{2d^2(\theta^*, \theta_0)} \right). \end{aligned}$$

By Lemma 2.2.1 of van der Vaart and Wellner (1996),

$$\|\mathbb{W}_{p_1 p_2 T}(\theta^*)\|_{\psi_2} \lesssim d(\theta^*, \theta_0) / \sqrt{p_1 p_2 T}. \quad (4)$$

Since  $\theta^*$  can take at most  $J_1^{p_1} J_2^{p_2} J_3^T \lesssim (K_1/\epsilon)^{k_1 p_1} (K_2/\epsilon)^{k_2 p_2} (K_3/\epsilon)^{k_1 k_2 T} \lesssim (K/\epsilon)^{k_1 p_1 + k_2 p_2 + k_1 k_2 T}$  different values, for some constant  $K$  and  $d(\theta^*, \theta_0) \lesssim K$ .

Lemma 2.2.2 of van der Vaart and Wellner (1996) shows that for any random variables  $X_1, \dots, X_m$ ,

$$\left\| \max_{1 \leq i \leq m} X_i \right\|_{\psi} \leq K \psi^{-1}(m) \max_i \|X_i\|_{\psi},$$

for a constant  $K$  depending only on a convex, nondecreasing, nonzero function  $\psi$ . Then, together with (4), we have

$$\begin{aligned} \mathbb{E} \left[ \sup_{\theta \in \Theta^{k_1 k_2}} |\mathbb{W}_{p_1 p_2 T}(\theta^*)| \right] &\leq \left\| \sup_{\theta \in \Theta^{k_1 k_2}} |\mathbb{W}_{p_1 p_2 T}(\theta^*)| \right\|_{\psi_2} \\ &\lesssim \sqrt{\log(K/\epsilon)} \sqrt{k_1 p_1 + k_2 p_2 + k_1 k_2 T} / \sqrt{p_1 p_2 T} \\ &\lesssim \sqrt{\log(K/\epsilon)} / L_{p_1 p_2 T}. \end{aligned} \quad (5)$$

Finally, by Markov's inequality and (3), for any  $\delta > 0$ ,

$$\begin{aligned} &P \left[ \sup_{\theta \in \Theta^{k_1 k_2}} |\mathbb{W}_{p_1 p_2 T}(\theta)| > \delta \right] \\ &\leq P \left[ \sup_{\theta \in \Theta^{k_1 k_2}} |\mathbb{W}_{p_1 p_2 T}(\theta^*)| > \delta/2 \right] + P \left[ \sup_{\theta \in \Theta^{k_1 k_2}} |\mathbb{W}_{p_1 p_2 T}(\theta) - \mathbb{W}_{p_1 p_2 T}(\theta^*)| > \delta/2 \right] \\ &\leq 2/\delta \mathbb{E} \left[ \sup_{\theta \in \Theta^{k_1 k_2}} |\mathbb{W}_{p_1 p_2 T}(\theta^*)| \right] + P[6\epsilon > \delta/2]. \end{aligned}$$

Thus, (2) follows from (5) since  $\epsilon$  is arbitrary. This concludes the proof.  $\square$

Define  $\Theta^{k_1 k_2}(\delta) = \{\theta \in \Theta^{k_1 k_2} : d(\theta, \theta_0) \leq \delta\}$ .

**Lemma B.2.** *Under Assumption 1 and for sufficiently small  $\delta > 0$ , for any  $\theta \in \Theta^{k_1 k_2}(\delta)$ , it holds that*

$$\|\mathbf{R} - \mathbf{R}_0\|_F / \sqrt{p_1} + \|\mathbf{F} - \mathbf{F}_0\|_F / \sqrt{T} + \|\mathbf{C} - \mathbf{C}_0\|_F / \sqrt{p_2} \leq K_7 d(\theta, \theta_0) \leq K_7 \delta.$$

*Proof.* Since  $\mathbf{R}'\mathbf{R}/p_1 = \mathbf{R}'_0\mathbf{R}_0/p_1 = \mathbb{I}_{k_1}$ ,  $\mathbf{C}'\mathbf{C}/p_2 = \mathbf{C}'_0\mathbf{C}_0/p_2 = \mathbb{I}_{k_2}$  and  $\|\mathbf{F}_0\|/\sqrt{T} \leq K_8$  by

Assumption 1-1, we have

$$\begin{aligned}
\|\mathbf{F} - \mathbf{F}_0\|_F/\sqrt{T} &= \sqrt{\sum_{t=1}^T \|\mathbf{F}_t - \mathbf{F}_{0t}\|_F^2/T} = \sqrt{\sum_{t=1}^T \|\mathbf{R}(\mathbf{F}_t - \mathbf{F}_{0t})\mathbf{C}'\|_F^2/p_1p_2T} \\
&= \sqrt{\sum_{t=1}^T \|\mathbf{R}\mathbf{F}_t\mathbf{C}' - \mathbf{R}_0\mathbf{F}_{0t}\mathbf{C}'_0 + \mathbf{R}_0\mathbf{F}_{0t}\mathbf{C}'_0 - \mathbf{R}\mathbf{F}_{0t}\mathbf{C}'_0 + \mathbf{R}\mathbf{F}_{0t}\mathbf{C}'_0 - \mathbf{R}\mathbf{F}_{0t}\mathbf{C}'\|_F^2/p_1p_2T} \\
&\leq \sqrt{3 \sum_{t=1}^T \frac{\|\mathbf{R}\mathbf{F}_t\mathbf{C}' - \mathbf{R}_0\mathbf{F}_{0t}\mathbf{C}'_0\|_F^2 + \|\mathbf{R}_0\mathbf{F}_{0t}\mathbf{C}'_0 - \mathbf{R}\mathbf{F}_{0t}\mathbf{C}'_0\|_F^2 + \|\mathbf{R}\mathbf{F}_{0t}\mathbf{C}'_0 - \mathbf{R}\mathbf{F}_{0t}\mathbf{C}'\|_F^2}{p_1p_2T}} \\
&\leq \sqrt{3} \left( d(\theta, \theta_0) + \sqrt{\frac{\|\mathbf{R} - \mathbf{R}_0\|_F^2}{p_1} \frac{\sum_{t=1}^T \|\mathbf{F}_{0t}\|_F^2}{T} \frac{\|\mathbf{C}'_0\|_F^2}{p_2}} + \sqrt{\frac{\|\mathbf{R}\|_F^2}{p_1} \frac{\sum_{t=1}^T \|\mathbf{F}_{0t}\|_F^2}{T} \frac{\|\mathbf{C}'_0 - \mathbf{C}'\|_F^2}{p_2}} \right) \\
&\leq \sqrt{3} \left( d(\theta, \theta_0) + \frac{\|\mathbf{R} - \mathbf{R}_0\|_F}{\sqrt{p_1}} K_8 \sqrt{k_2} + \sqrt{k_1} K_8 \frac{\|\mathbf{C}'_0 - \mathbf{C}'\|_F}{\sqrt{p_2}} \right)
\end{aligned}$$

Thus, for  $\theta \in \Theta^{k_1 k_2}(\delta)$ ,

$$\begin{aligned}
&\frac{\|\mathbf{F} - \mathbf{F}_0\|_F}{\sqrt{T}} + \frac{\|\mathbf{R} - \mathbf{R}_0\|_F}{\sqrt{p_1}} + \frac{\|\mathbf{C} - \mathbf{C}_0\|_F}{\sqrt{p_2}} \\
&\leq \sqrt{3}\delta + (1 + K_8\sqrt{k_2}) \frac{\|\mathbf{R} - \mathbf{R}_0\|_F}{\sqrt{p_1}} + (1 + K_8\sqrt{k_1}) \frac{\|\mathbf{C} - \mathbf{C}_0\|_F}{\sqrt{p_2}}.
\end{aligned} \tag{6}$$

Second,

$$\begin{aligned}
&\|\mathbf{C} - \mathbf{C}_0\|_F/\sqrt{p_2} \\
&= \|\mathbf{C}_0 - \mathbf{C}(\mathbf{C}'\mathbf{C}_0/p_2) + \mathbf{C}(\mathbf{C}'\mathbf{C}_0/p_2) - \mathbf{C}\|_F/\sqrt{p_2} \\
&\leq \|\mathbf{C}_0 - \mathbf{C}(\mathbf{C}'\mathbf{C}_0/p_2)\|_F/\sqrt{p_2} + \|\mathbf{C}(\mathbf{C}'\mathbf{C}_0/p_2) - \mathbf{C}\|_F/\sqrt{p_2} \\
&= \|M_c\mathbf{C}_0\|_F/\sqrt{p_2} + \|\mathbf{C}'\mathbf{C}_0/p_2 - \mathbb{I}_{k_2}\|_F,
\end{aligned} \tag{7}$$

where  $M_A = \mathbb{I} - P_A$  and  $P_A = A(A'A)^{-1}A'$ .

Third,

$$\begin{aligned}
&\sqrt{\sum_{t=1}^T \|(\mathbf{R}\mathbf{F}_t\mathbf{C}' - \mathbf{R}_0\mathbf{F}_{0t}\mathbf{C}'_0)M_c\|_F^2/p_1p_2T} \\
&\leq \sqrt{\sum_{t=1}^T \text{rank}[(\mathbf{R}\mathbf{F}_t\mathbf{C}' - \mathbf{R}_0\mathbf{F}_{0t}\mathbf{C}'_0)M_c] \|M_c\|_S^2 \|\mathbf{R}\mathbf{F}_t\mathbf{C}' - \mathbf{R}_0\mathbf{F}_{0t}\mathbf{C}'_0\|_S^2/p_1p_2T}
\end{aligned}$$

$$\lesssim \sqrt{\sum_{t=1}^T \|\mathbf{R}\mathbf{F}_t\mathbf{C}' - \mathbf{R}_0\mathbf{F}_{0t}\mathbf{C}'_0\|_F^2/p_1p_2T} = d(\theta, \theta_0). \quad (8)$$

Since  $\mathbf{R}'_0\mathbf{R}_0/p_1 = \mathbb{I}_{k_1}$ , then  $\sum_{t=1}^T \mathbf{F}'_{0t}\mathbf{R}'_0\mathbf{R}_0\mathbf{F}_{0t}/p_1T = \sum_{t=1}^T \mathbf{F}'_{0t}\mathbf{F}_{0t}/T$ . By Assumption 1-1, we have  $\frac{1}{T} \sum_{t=1}^T \mathbf{F}'_{0t}\mathbf{F}_{0t} = \text{diag}(\sigma'_{T_1}, \dots, \sigma'_{T_{k_2}})$  with  $\sigma'_{T_1} \geq \dots \geq \sigma'_{T_{k_2}}$ . Thus,

$$\text{Tr}\left[\left(\sum_{t=1}^T \mathbf{F}'_{0t}\mathbf{R}'_0\mathbf{R}_0\mathbf{F}_{0t}/p_1T\right)(\mathbf{C}'_0M_C\mathbf{C}_0/p_2)\right] \geq \sigma'_{T_{k_2}} \text{Tr}(\mathbf{C}'_0M_C\mathbf{C}_0/p_2).$$

We have

$$\begin{aligned} & \sqrt{\sum_{t=1}^T \|(\mathbf{R}\mathbf{F}_t\mathbf{C}' - \mathbf{R}_0\mathbf{F}_{0t}\mathbf{C}'_0)M_C\|_F^2/p_1p_2T} \\ &= \sqrt{\sum_{t=1}^T \|\mathbf{R}_0\mathbf{F}_{0t}\mathbf{C}'_0M_C\|_F^2/p_1p_2T} \\ &= \sqrt{\text{Tr}\left[\left(\sum_{t=1}^T \mathbf{F}'_{0t}\mathbf{R}'_0\mathbf{R}_0\mathbf{F}_{0t}/p_1T\right)(\mathbf{C}'_0M_C\mathbf{C}_0/p_2)\right]} \\ &\geq \sqrt{\sigma'_{T_{k_2}}} \cdot \sqrt{\text{Tr}(\mathbf{C}'_0M_C\mathbf{C}_0/p_2)} = \sqrt{\sigma'_{T_{k_2}}} \|\mathbf{M}_C\mathbf{C}_0\|_F/\sqrt{p_2}. \end{aligned} \quad (9)$$

It follows from (8) and (9) that

$$\|\mathbf{M}_C\mathbf{C}_0\|_F/\sqrt{p_2} \lesssim \sqrt{\frac{1}{\sigma'_{T_{k_2}}}} d(\theta, \theta_0). \quad (10)$$

Similarly, it can be shown that

$$\|\mathbf{M}_{C_0}\mathbf{C}\|_F/\sqrt{p_2} \lesssim \sqrt{\frac{1}{\rho_{\min}\left(\sum_{t=1}^T \mathbf{F}'_t\mathbf{R}'\mathbf{R}\mathbf{F}_t/Tp_1\right)}} d(\theta, \theta_0). \quad (11)$$

where  $\rho_{\min}$  denotes the minimum eigenvalue.

Fourth, we have

$$\begin{aligned} & \sqrt{\sum_{t=1}^T \|(\mathbf{R}\mathbf{F}_t\mathbf{C}' - \mathbf{R}_0\mathbf{F}_{0t}\mathbf{C}'_0)P_c\|_F^2/p_1p_2T} \\ &\leq \sqrt{\sum_{t=1}^T \|(\mathbf{R}\mathbf{F}_t\mathbf{C}' - \mathbf{R}_0\mathbf{F}_{0t}\mathbf{C}'_0)\|_F^2\|P_c\|_F^2/p_1p_2T} \\ &= d(\theta, \theta_0)\|P_c\|_F = \sqrt{k_2}d(\theta, \theta_0), \end{aligned}$$

so

$$\begin{aligned}
& \frac{1}{\sqrt{p_1 T}} \sqrt{\sum_{t=1}^T \|\mathbf{R}\mathbf{F}_t - \mathbf{R}_0 \mathbf{F}_{0t}(\mathbf{C}'_0 \mathbf{C}/p_2)\|_F^2} \\
&= \frac{1}{\sqrt{p_1 p_2 T}} \sqrt{\sum_{t=1}^T \|\mathbf{R}\mathbf{F}_t \mathbf{C}' - \mathbf{R}_0 \mathbf{F}_{0t}(\mathbf{C}'_0 \mathbf{C}/p_2) \mathbf{C}'\|_F^2} \\
&= \frac{1}{\sqrt{p_1 p_2 T}} \sqrt{\sum_{t=1}^T \|(\mathbf{R}\mathbf{F}_t \mathbf{C}' - \mathbf{R}_0 \mathbf{F}_{0t} \mathbf{C}'_0) P_c\|_F^2} \\
&\leq \sqrt{k_2} d(\theta, \theta_0).
\end{aligned} \tag{12}$$

Likewise, it can be shown that

$$\frac{1}{\sqrt{p_1 T}} \sqrt{\sum_{t=1}^T \|\mathbf{R}_0 \mathbf{F}_{0t} - \mathbf{R}\mathbf{F}_t(\mathbf{C}' \mathbf{C}_0/p_2)\|_F^2} \leq \sqrt{k_2} d(\theta, \theta_0). \tag{13}$$

Fifth, define  $\mathbf{R}_{p_2} = \mathbf{C}' \mathbf{C}_0/p_2$ . Note that  $\mathbf{C} \mathbf{R}_{p_2} = \mathbf{C} \mathbf{C}' \mathbf{C}_0/p_2 = P_C \mathbf{C}_0$ , thus

$$\begin{aligned}
\mathbb{I}_{k_2} &= \mathbf{C}'_0 \mathbf{C}_0/p_2 = \mathbf{R}'_{p_2}(\mathbf{C}' \mathbf{C}/p_2) \mathbf{R}_{p_2} + \mathbf{C}'_0 \mathbf{C}_0/p_2 - \mathbf{R}'_{p_2}(\mathbf{C}' \mathbf{C}/p_2) \mathbf{R}_{p_2} \\
&= \mathbf{R}'_{p_2} \mathbf{R}_{p_2} + \mathbf{C}'_0 \mathbf{C}_0/p_2 - \mathbf{C}'_0 \mathbf{C} \mathbf{R}_{p_2}/p_2 + \mathbf{C}'_0 \mathbf{C} \mathbf{R}_{p_2}/p_2 - \mathbf{R}'_{p_2}(\mathbf{C}' \mathbf{C}/p_2) \mathbf{R}_{p_2} \\
&= \mathbf{R}'_{p_2} \mathbf{R}_{p_2} + \mathbf{C}'_0(\mathbf{C}_0 - \mathbf{C} \mathbf{R}_{p_2})/p_2 = \mathbf{R}'_{p_2} \mathbf{R}_{p_2} + \mathbf{C}'_0 M_C \mathbf{C}_0/p_2,
\end{aligned} \tag{14}$$

because

$$\mathbf{C}'_0 \mathbf{C} \mathbf{R}_{p_2}/p_2 - \mathbf{R}'_{p_2}(\mathbf{C}' \mathbf{C}/p_2) \mathbf{R}_{p_2} = (\mathbf{C}_0 - \mathbf{C} \mathbf{R}_{p_2})' \mathbf{C} \mathbf{R}_{p_2}/p_2 = \mathbf{C}'_0 M_C \mathbf{C} \mathbf{R}_{p_2}/p_2 = 0.$$

In addition,

$$\begin{aligned}
& \sum_{t=1}^T (\mathbf{R}_0 \mathbf{F}_{0t})' \mathbf{R}_0 \mathbf{F}_{0t}/p_1 T \\
&= \mathbf{R}'_{p_2} \left( \sum_{t=1}^T \mathbf{F}'_t \mathbf{R}' \mathbf{R} \mathbf{F}_t/p_1 T \right) \mathbf{R}_{p_2} \\
&\quad + \left( \sum_{t=1}^T \mathbf{F}'_{0t} \mathbf{R}'_0 \mathbf{R}_0 \mathbf{F}_{0t}/p_1 T - \mathbf{R}'_{p_2} \left( \sum_{t=1}^T \mathbf{F}'_t \mathbf{R}' \mathbf{R} \mathbf{F}_t/p_1 T \right) \mathbf{R}_{p_2} \right) \\
&= \mathbf{R}'_{p_2} \left( \sum_{t=1}^T \mathbf{F}'_t \mathbf{R}' \mathbf{R} \mathbf{F}_t/p_1 T \right) \mathbf{R}_{p_2} + \sum_{t=1}^T \mathbf{F}'_{0t} \mathbf{R}'_0 (\mathbf{R}_0 \mathbf{F}_{0t} - \mathbf{R} \mathbf{F}_t \mathbf{R}_{p_2})/p_1 T \\
&\quad + \sum_{t=1}^T (\mathbf{R}_0 \mathbf{F}_{0t} - \mathbf{R} \mathbf{F}_t \mathbf{R}_{p_2})' \mathbf{R} \mathbf{F}_t \mathbf{R}_{p_2}/p_1 T.
\end{aligned} \tag{15}$$

Similar to the proof of (14), we have

$$\mathbb{I}_{k_2} = \mathbf{R}_{p_2} \mathbf{R}'_{p_2} + \mathbf{C}'(\mathbf{C} - \mathbf{C}_0 \mathbf{R}'_{p_2})/p_2 = \mathbf{R}_{p_2} \mathbf{R}'_{p_2} + \mathbf{C}' M_{C_0} \mathbf{C}/p_2. \quad (16)$$

From (15), it holds that

$$\begin{aligned} & \sum_{t=1}^T \mathbf{F}'_{0t} \mathbf{R}'_0 \mathbf{R}_0 \mathbf{F}_{0t} / p_1 T \\ &= \mathbf{R}'_{p_2} \left( \sum_{t=1}^T \mathbf{F}'_t \mathbf{R}' \mathbf{R} \mathbf{F}_t / p_1 T \right) (\mathbf{R}'_{p_2})^{-1} \mathbf{R}'_{p_2} \mathbf{R}_{p_2} \\ & \quad + \sum_{t=1}^T \mathbf{F}'_{0t} \mathbf{R}'_0 (\mathbf{R}_0 \mathbf{F}_{0t} - \mathbf{R} \mathbf{F}_t \mathbf{R}_{p_2}) / p_1 T + \sum_{t=1}^T (\mathbf{R}_0 \mathbf{F}_{0t} - \mathbf{R} \mathbf{F}_t \mathbf{R}_{p_2})' \mathbf{R} \mathbf{F}_t \mathbf{R}_{p_2} / p_1 T \\ &= \mathbf{R}'_{p_2} \left( \sum_{t=1}^T \mathbf{F}'_t \mathbf{R}' \mathbf{R} \mathbf{F}_t / p_1 T \right) (\mathbf{R}'_{p_2})^{-1} + \mathbf{R}'_{p_2} \left( \sum_{t=1}^T \mathbf{F}'_t \mathbf{R}' \mathbf{R} \mathbf{F}_t / p_1 T \right) (\mathbf{R}'_{p_2})^{-1} (\mathbf{R}'_{p_2} \mathbf{R}_{p_2} - \mathbb{I}_{k_2}) \\ & \quad + \sum_{t=1}^T \mathbf{F}'_{0t} \mathbf{R}'_0 (\mathbf{R}_0 \mathbf{F}_{0t} - \mathbf{R} \mathbf{F}_t \mathbf{R}_{p_2}) / p_1 T + \sum_{t=1}^T (\mathbf{R}_0 \mathbf{F}_{0t} - \mathbf{R} \mathbf{F}_t \mathbf{R}_{p_2})' \mathbf{R} \mathbf{F}_t \mathbf{R}_{p_2} / p_1 T, \end{aligned}$$

and then it follows from the above equation and (14) that

$$\left( \sum_{t=1}^T \mathbf{F}'_{0t} \mathbf{R}'_0 \mathbf{R}_0 \mathbf{F}_{0t} / p_1 T + D_{p_1 p_2 T} \right) \mathbf{R}'_{p_2} = \mathbf{R}'_{p_2} \left( \sum_{t=1}^T \mathbf{F}'_t \mathbf{R}' \mathbf{R} \mathbf{F}_t / p_1 T \right), \quad (17)$$

where

$$\begin{aligned} D_{p_1 p_2 T} &= \mathbf{R}'_{p_2} \left( \sum_{t=1}^T \mathbf{F}'_t \mathbf{R}' \mathbf{R} \mathbf{F}_t / p_1 T \right) (\mathbf{R}'_{p_2})^{-1} \mathbf{C}'_0 M_C \mathbf{C}_0 / p_2 \\ & \quad - \sum_{t=1}^T \mathbf{F}'_{0t} \mathbf{R}'_0 (\mathbf{R}_0 \mathbf{F}_{0t} - \mathbf{R} \mathbf{F}_t \mathbf{R}_{p_2}) / p_1 T - \sum_{t=1}^T (\mathbf{R}_0 \mathbf{F}_{0t} - \mathbf{R} \mathbf{F}_t \mathbf{R}_{p_2})' \mathbf{R} \mathbf{F}_t \mathbf{R}_{p_2} / p_1 T. \end{aligned}$$

From (10), (12) and (13), we have that  $\|D_{p_1 p_2 T}\|_F \lesssim d(\theta, \theta_0)$ .

By the Bauer-Fike theorem and  $\|X\|_S \leq \|X\|_F$ , it holds that

$$\begin{aligned} & \left| \rho_{\min} \left[ \sum_{t=1}^T \mathbf{F}'_t \mathbf{R}' \mathbf{R} \mathbf{F}_t / p_1 T \right] - \rho_{\min} \left[ \sum_{t=1}^T \mathbf{F}'_{0t} \mathbf{R}'_0 \mathbf{R}_0 \mathbf{F}_{0t} / p_1 T \right] \right| \leq \|D_{p_1 p_2 T}\|_S \\ & \leq \|D_{p_1 p_2 T}\|_F \lesssim d(\theta, \theta_0). \end{aligned} \quad (18)$$

Moreover, by Assumption 1-1 and the perturbation theory for eigenvectors (see Section 6.12 of Franklin (2012)),

$$\|\mathbf{R}'_{p_2} V_{p_2} - \mathbb{I}_{k_2}\|_F \lesssim d(\theta, \theta_0), \quad (19)$$

where  $V_{p_2} = \text{diag}((\mathbf{R}_{p_2,1}, \mathbf{R}'_{p_2,1})^{-\frac{1}{2}}, \dots, (\mathbf{R}_{p_2,k_2}, \mathbf{R}'_{p_2,k_2})^{-\frac{1}{2}})$ , and  $\mathbf{R}'_{p_2,j}$  is the  $j$ th column of  $\mathbf{R}'_{p_2}$ .

Furthermore, (11) and (18) imply that  $\rho_{\min} \left[ \sum_{t=1}^T \mathbf{F}'_t \mathbf{R}' \mathbf{R} \mathbf{F}_t / p_1 T \right]$  is bounded below by a positive constant, and that

$$\|M_{C_0} \mathbf{C}\|_F / \sqrt{p_2} \lesssim d(\theta, \theta_0). \quad (20)$$

Note that the triangular inequality implies that

$$\|\mathbf{R}'_{p_2} - \mathbb{I}_{k_2}\|_F \leq \|\mathbf{R}'_{p_2} V_{p_2} - \mathbb{I}_{k_2}\|_F + \|\mathbf{R}'_{p_2} V_{p_2} - \mathbf{R}_{p_2}\|_F \leq \|\mathbf{R}'_{p_2} V_{p_2} - \mathbb{I}_{k_2}\|_F + \|\mathbf{R}_{p_2}\|_F \|V_{p_2} - \mathbb{I}_{k_2}\|_F. \quad (21)$$

From (16) and (20), we get

$$\|V_{p_2} - \mathbb{I}_{k_2}\|_F \lesssim \|\mathbf{R}_{p_2} \mathbf{R}'_{p_2} - \mathbb{I}_{k_2}\|_F = \|\mathbf{C}' M_{C_0} \mathbf{C} / p_2\|_F = \|M_{C_0} \mathbf{C}\|_F^2 / p_2 \lesssim d^2(\theta, \theta_0). \quad (22)$$

For small enough  $d(\theta, \theta_0)$ , it then follows from (19), (21), and (22) that

$$\|\mathbf{C}' \mathbf{C}_0 / p_2 - \mathbb{I}_{k_2}\|_F = \|\mathbf{R}_{p_2} - \mathbb{I}_{k_2}\|_F \lesssim d(\theta, \theta_0). \quad (23)$$

Finally, it follows from (7), (10), and (23) that for sufficiently small  $d(\theta, \theta_0)$ ,

$$\|\mathbf{C} - \mathbf{C}_0\|_F / \sqrt{p_2} \lesssim d(\theta, \theta_0). \quad (24)$$

Similarly, we can also get

$$\|\mathbf{R} - \mathbf{R}_0\|_F / \sqrt{p_1} \lesssim d(\theta, \theta_0). \quad (25)$$

Then the desired result follows from (6), (24) and (25).  $\square$

**Lemma B.3.** *Under Assumption 1, for sufficiently small  $\delta$ , it holds that*

$$\mathbb{E} \left[ \sup_{\theta \in \Theta^{k_1 k_2}(\delta)} |\mathbb{W}_{p_1 p_2 T}(\theta)| \right] \lesssim \frac{\delta}{L_{p_1 p_2 T}}.$$

*Proof.* In the proof of Lemma B.1 we have shown that, for  $\theta_a, \theta_b \in \Theta^{k_1 k_2}$ ,

$$\|\sqrt{p_1 p_2 T} |\mathbb{W}_{p_1 p_2 T}(\theta_a) - \mathbb{W}_{p_1 p_2 T}(\theta_b)|\|_{\psi_2} \lesssim d(\theta_a, \theta_b). \quad (26)$$

Since the process  $\mathbb{W}_{p_1 p_2 T}(\theta)$  is separable, it follows from Theorem 2.2.4 of van der Vaart and Wellner (1996) that

$$\mathbb{E} \left[ \sup_{\theta \in \Theta^{k_1 k_2}(\delta)} |\mathbb{W}_{p_1 p_2 T}(\theta)| \right] \lesssim \sup_{\theta \in \Theta^{k_1 k_2}(\delta)} \|\mathbb{W}_{p_1 p_2 T}(\theta)\|_{\psi_2} \lesssim \int_0^\delta \sqrt{\log D(\epsilon, d, \theta \in \Theta^{k_1 k_2}(\delta))} d\epsilon.$$

Thus, it remains to show that

$$\int_0^\delta \sqrt{\log D(\epsilon, d, \theta \in \Theta^{k_1 k_2}(\delta))} d\epsilon = O(\sqrt{k_1 p_1 + k_2 p_2 + T p_1 p_2 \delta}). \quad (27)$$

To prove (27), first note that Lemma B.2 implies that

$$\Theta^{k_1 k_2}(\delta) \subset \Theta_S^{k_1 k_2}(\delta),$$

where  $\Theta_S^{k_1 k_2}(\delta) = \{\theta \in \Theta^{k_1 k_2} : \|\mathbf{R} - \mathbf{R}_0\|_F / \sqrt{p_1} + \|\mathbf{F} - \mathbf{F}_0\|_F / \sqrt{T} + \|\mathbf{C} - \mathbf{C}_0\|_F / \sqrt{p_2} \leq K_7 \delta\}$ . It suffices to show that

$$\int_0^\delta \sqrt{\log D(\epsilon, d, \Theta_S^{k_1 k_2}(\delta))} d\epsilon = O(\sqrt{k_1 p_1 + k_2 p_2 + T p_1 p_2 \delta}).$$

Second, for any  $\theta_a, \theta_b \in \Theta^{k_1 k_2}$ ,

$$\begin{aligned} d(\theta_a, \theta_b) &= \frac{1}{\sqrt{p_1 p_2 T}} \sqrt{\sum_{t=1}^T \|\mathbf{R}_a \mathbf{F}_{at} \mathbf{C}'_a - \mathbf{R}_b \mathbf{F}_{bt} \mathbf{C}'_b\|_F^2} \\ &= \frac{1}{\sqrt{p_1 p_2 T}} \sqrt{\sum_{t=1}^T \|\mathbf{R}_a \mathbf{F}_{at} \mathbf{C}'_a - \mathbf{R}_b \mathbf{F}_{at} \mathbf{C}'_a + \mathbf{R}_b \mathbf{F}_{at} \mathbf{C}'_a - \mathbf{R}_b \mathbf{F}_{bt} \mathbf{C}'_a + \mathbf{R}_b \mathbf{F}_{bt} \mathbf{C}'_a - \mathbf{R}_b \mathbf{F}_{bt} \mathbf{C}'_b\|_F^2} \\ &\leq \frac{\sqrt{3}}{\sqrt{p_1 p_2 T}} (\|\mathbf{R}_a - \mathbf{R}_b\|_F \|\mathbf{F}_a\|_F \|\mathbf{C}'_a\|_F + \|\mathbf{R}_b\|_F \|\mathbf{F}_a - \mathbf{F}_b\|_F \|\mathbf{C}'_a\|_F \\ &\quad + \|\mathbf{R}_b\|_F \|\mathbf{F}_b\|_F \|\mathbf{C}'_a - \mathbf{C}'_b\|_F) \\ &\leq K_8 \left( \frac{\|\mathbf{R}_a - \mathbf{R}_b\|_F}{\sqrt{p_1}} + \frac{\|\mathbf{F}_a - \mathbf{F}_b\|_F}{\sqrt{T}} + \frac{\|\mathbf{C}'_a - \mathbf{C}'_b\|_F}{\sqrt{p_2}} \right), \end{aligned}$$

where  $K_8 \geq 1$ . Now define

$$d^*(\theta_a, \theta_b) = 3K_9 \sqrt{\frac{\|\mathbf{R}_a - \mathbf{R}_b\|_F^2}{p_1} + \frac{\|\mathbf{F}_a - \mathbf{F}_b\|_F^2}{T} + \frac{\|\mathbf{C}'_a - \mathbf{C}'_b\|_F^2}{p_2}}.$$

It follows from  $\sqrt{a} + \sqrt{b} + \sqrt{c} \leq 3\sqrt{a+b+c}$  that  $d(\theta_a, \theta_b) \leq d^*(\theta_a, \theta_b)$ . Moreover, it follows from  $\sqrt{a+b+c} \leq \sqrt{a} + \sqrt{b} + \sqrt{c}$  that  $\Theta_S^{k_1 k_2}(\delta) \subset \Theta^{k_1 k_2*}(\delta) = \{\theta \in \Theta^{k_1 k_2} : d^*(\theta, \theta_0) \leq K_{10}\delta\}$ , where  $K_{10} = 3K_7K_9$ .

Let  $(T, d)$  be a semimetric space. Then, for any  $S \subset T$ , it can be shown that  $D(\epsilon, d, S) \leq D(\epsilon/2, d, T) \leq C(\epsilon/4, d, T)$ . It then follows that

$$\begin{aligned} D(\epsilon, d, \Theta_S^{k_1 k_2}(\delta)) &\leq D(\epsilon, d^*, \Theta_S^{k_1 k_2}(\delta)) \leq D(\epsilon/2, d^*, \Theta^{k_1 k_2*}(\delta)) \\ &\leq C(\epsilon/4, d^*, \Theta^{k_1 k_2*}(\delta)). \end{aligned} \quad (28)$$

Next, we find an upper bound for  $C(\epsilon/4, d^*, \Theta^{k_1 k_2*}(\delta))$  as follows. Let  $\eta = \epsilon/4$ , and  $\theta_1^*, \dots, \theta_J^*$  be a maximal set in  $\Theta^{k_1 k_2*}(\delta)$  such that  $d^*(\theta_j^*, \theta_l^*) > \eta$  for any  $j \neq l$ . Define  $B(\theta, c) = \{\gamma \in \Theta^{k_1 k_2} : d^*(\gamma, \theta) \leq c\}$ . Then the balls  $B(\theta_1^*, \eta), \dots, B(\theta_J^*, \eta)$  over  $\Theta^{k_1 k_2*}(\delta)$  and thus  $C(\epsilon/4, d^*, \Theta^{k_1 k_2*}(\delta)) \leq J$ . Moreover, the balls  $B(\theta_1^*, \eta/4), \dots, B(\theta_J^*, \eta/4)$  are disjoint and

$$\bigcup_{j=1}^J B(\theta_j^*, \eta/4) \subset \Theta^{k_1 k_2*}(\delta + \eta/4).$$

Note that the volume of a ball defined by the metric  $d^*$  with radius  $c$  is the volume of an ellipsoid, which is equal to  $h_M \cdot c^M$ , where  $h_M$  is a constant that depends on  $p_1, p_2, T$  and  $k_1, k_2$ , but not on  $c$ . Therefore, we have

$$J \cdot h_M \cdot (\eta/4)^M \leq h_M \cdot (K_{10}(\delta + \eta/4))^M,$$

which implies

$$J \leq \left( \frac{K_{10}(4\delta + \eta)}{\eta} \right)^M = \left( \frac{K_{10}(16\delta + \epsilon)}{\epsilon} \right)^M \leq \left( \frac{K_{11}\delta}{\epsilon} \right)^M \quad (29)$$

for  $\epsilon \leq \delta$ . It then follows from (28) and (29) that

$$\begin{aligned} \int_0^\delta \sqrt{\log D(\epsilon, d, \Theta_S^{k_1 k_2}(\delta))} d\epsilon &\leq \int_0^\delta \sqrt{C(\epsilon/4, d^*, \Theta^{k_1 k_2*}(\delta))} d\epsilon \\ &\leq \sqrt{k_1 p_1 + k_2 p_2 + T p_1 p_2} \int_0^\delta \sqrt{\log(K_{11}\delta/\epsilon)} d\epsilon. \end{aligned}$$

It is easy to show that  $\int_0^\delta \sqrt{\log(K_{11}\delta/\epsilon)} d\epsilon = O(\delta)$  and thus (27) follows. This concludes the proof of Lemma B.3.  $\square$

### B.3 Proof of Theorem 3.2

The parameter space  $\Theta^{k_1 k_2}$  can be partitioned into shells  $S_j = \{\theta \in \Theta^{k_1 k_2} : 2^{j-1} < L_{p_1 p_2 T} \cdot d(\theta, \theta_0) \leq 2^j\}$ . If  $L_{p_1 p_2 T} \cdot d(\hat{\theta}, \theta_0)$  is larger than  $2^V$  for a given integer  $V$ , then  $\hat{\theta}$  is in one of the shells  $S_j$  with  $j > V$ . In such a case, the infimum of the mapping  $\theta \mapsto \mathbb{M}_{p_1 p_2 T}^*(\theta) = \mathbb{M}_{p_1 p_2 T}(\theta) - \mathbb{M}_{p_1 p_2 T}(\theta_0)$  over this shell is nonpositive by the definition of  $\hat{\theta}$ . From this we conclude that, for every  $\eta > 0$ ,

$$P[L_{p_1 p_2 T} \cdot d(\hat{\theta}, \theta_0) > 2^V] \leq \sum_{j > V, 2^{j-1} \leq \eta L_{p_1 p_2 T}} P\left[\inf_{\theta \in S_j} \mathbb{M}_{p_1 p_2 T}^*(\theta) \leq 0\right] + P[d(\hat{\theta}, \theta_0) > \eta].$$

For arbitrarily small  $\eta > 0$ , the second probability on the RHS of the above equation converges to 0 as  $p_1, p_2, T \rightarrow \infty$  by Lemma B.1.

Next, note that by (1), for each  $\theta$  in  $S_j$  we have

$$-\bar{\mathbb{M}}_{p_1 p_2 T}^*(\theta) \lesssim -d^2(\theta, \theta_0) \leq -\frac{2^{2j-2}}{L_{p_1 p_2 T}^2}.$$

Thus,  $\inf_{\theta \in S_j} \mathbb{M}_{p_1 p_2 T}^*(\theta) \leq 0$  implies that

$$\inf_{\theta \in S_j} \mathbb{W}_{p_1 p_2 T}(\theta) \leq -\frac{2^{2j-2}}{L_{p_1 p_2 T}^2},$$

and therefore,

$$\sum_{j > V, 2^{j-1} \leq \eta L_{p_1 p_2 T}} P\left[\inf_{\theta \in S_j} \mathbb{M}_{p_1 p_2 T}^*(\theta) \leq 0\right] \leq \sum_{j > V, 2^{j-1} \leq \eta L_{p_1 p_2 T}} P\left[\sup_{\theta \in S_j} |\mathbb{W}_{p_1 p_2 T}(\theta)| \geq \frac{2^{2j-2}}{L_{p_1 p_2 T}^2}\right].$$

By Lemma B.3 and Markov's inequality, we have

$$P\left[\sup_{\theta \in S_j} |\mathbb{W}_{p_1 p_2 T}(\theta)| \geq \frac{2^{2j-2}}{L_{p_1 p_2 T}^2}\right] \lesssim \frac{L_{p_1 p_2 T}^2}{2^{2j}} \mathbb{E}\left[\sup_{\theta \in S_j} |\mathbb{W}_{p_1 p_2 T}(\theta)|\right] \lesssim \frac{L_{p_1 p_2 T}^2}{2^{2j}} \frac{2^{j\alpha}}{L_{p_1 p_2 T}^2} = 2^{j\alpha-2j},$$

for some  $1 < \alpha < 2$  according to Theorem 3.2.5 of van der Vaart and Wellner (1996). This implies that

$$\sum_{j > V, 2^{j-1} \leq \eta L_{p_1 p_2 T}} P\left[\inf_{\theta \in S_j} \mathbb{M}_{p_1 p_2 T}^*(\theta) \leq 0\right] \lesssim \sum_{j > V} 2^{j\alpha-2j}.$$

The RHS of the previous expression converges to 0 as  $V \rightarrow \infty$ , implying that  $L_{p_1 p_2 T} \cdot d(\hat{\theta}, \theta_0) = O_p(1)$ , or  $d(\hat{\theta}, \theta_0) = O_p(1/L_{p_1 p_2 T})$ . The desired result then follows from Lemma B.2.  $\square$

## C Proof of Theorem 4.1

This section provides the detailed technical proof of Theorem 4.1.

### C.1 Definitions and Notations

With a little abuse of notation, for  $\theta_a \in \Theta^{K_1 K_2}$  and  $\theta_b \in \Theta^{k_1 k_2}$ , let

$$d(\theta_a, \theta_b) = \sqrt{\sum_{t=1}^T \|\mathbf{R}_a \mathbf{F}_{at} \mathbf{C}'_a - \mathbf{R}_b \mathbf{F}_{bt} \mathbf{C}'_b\|^2 / \sqrt{p_1 p_2 T}}.$$

In this case,  $d$  is not a strict metric because  $\theta_a$  and  $\theta_b$  belong to different spaces.

For sufficiently small  $\delta$ , define  $\Theta^{K_1 K_2}(\delta) = \{\theta^{K_1 K_2} \in \Theta^{K_1 K_2} : d(\theta^{K_1 K_2}, \theta_0) \leq \delta\}$ . Let  $\mathbf{R}^{K_1, k_1}$  denote the first  $k_1$  columns of  $\mathbf{R}^{K_1}$ , and let  $\mathbf{R}^{K_1, -k_1}$  denote the remaining  $K_1 - k_1$  columns of  $\mathbf{R}^{K_1}$ .  $\mathbf{C}^{K_2, k_2}$  and  $\mathbf{C}^{K_2, -k_2}$  are defined similarly. Let  $\mathbf{F}_t^{K_1 \times K_2, k_1 \times k_2}$  denote the first  $k_1$  rows and  $k_2$  columns of  $\mathbf{F}_t^{K_1 \times K_2}$ , and let  $\mathbf{F}_t^{K_1 \times K_2, -(k_1 \times k_2)}$  denote the remaining  $K_1 - k_1$  rows and  $K_2 - k_2$  columns of  $\mathbf{F}_t^{K_1 \times K_2}$ , for  $t = 1, \dots, T$ . Let  $\mathbf{F}_t^{K_1 \times K_2, k_1 \times (-k_2)}$  denote the first  $k_1$  rows and the remaining  $K_2 - k_2$  columns of  $\mathbf{F}_t^{K_1 \times K_2}$  and  $\mathbf{F}_t^{K_1 \times K_2, (-k_1) \times k_2}$  denote the remaining  $K_1 - k_1$  rows and the first  $k_2$  columns of  $\mathbf{F}_t^{K_1 \times K_2}$ . Let  $\mathbf{F}^{K_1 \times K_2, k_1 \times k_2} = (\mathbf{F}_1^{K_1 \times K_2, k_1 \times k_2}, \dots, \mathbf{F}_T^{K_1 \times K_2, k_1 \times k_2})$ .

For any  $\theta^{K_1 K_2} \in \Theta^{K_1 K_2}$ , write

$$\begin{aligned} \mathbb{M}_{p_1 p_2 T}^*(\theta^{K_1 K_2}) &= \frac{1}{p_1 p_2 T} \sum_{i=1}^{p_1} \sum_{j=1}^{p_2} \sum_{t=1}^T [\rho_\tau(X_{ijt} - r_i^{K_1'} \mathbf{F}_t^{K_1 \times K_2} c_j^{K_2}) - \rho_\tau(X_{ijt} - r'_{0i} \mathbf{F}_{0t} c_{0j})], \\ \bar{\mathbb{M}}_{p_1 p_2 T}^*(\theta^{K_1 K_2}) &= \frac{1}{p_1 p_2 T} \sum_{i=1}^{p_1} \sum_{j=1}^{p_2} \sum_{t=1}^T \mathbb{E}[\rho_\tau(X_{ijt} - r_i^{K_1'} \mathbf{F}_t^{K_1 \times K_2} c_j^{K_2}) - \rho_\tau(X_{ijt} - r'_{0i} \mathbf{F}_{0t} c_{0j})], \\ \mathbb{W}_{p_1 p_2 T}(\theta^{K_1 K_2}) &= \mathbb{M}_{p_1 p_2 T}^*(\theta^{K_1 K_2}) - \bar{\mathbb{M}}_{p_1 p_2 T}^*(\theta^{K_1 K_2}). \end{aligned}$$

### C.2 Three Preliminary Lemmas

This subsection presents three preliminary lemmas to prove the Theorem 4.1.

**Lemma C.1.** Suppose that Assumption 1 holds and  $k_1 < K_1 < \infty$ ,  $k_2 < K_2 < \infty$ . Then  $d(\widehat{\theta}^{K_1 K_2}, \theta_0) = o_p(1)$ , as  $p_1, p_2, T \rightarrow \infty$ .

*Proof.* Note that  $\widehat{\theta}^{K_1 K_2}$  is obtained from the same check loss function as  $\widehat{\theta}^{k_1 k_2}$  by replacing the dimension of  $r_i, \mathbf{F}_t, c_j$  to  $K_1, K_1 \times K_2, K_2$ . The proof follows from two main results.

Firstly, a Taylor expansion of  $\bar{\mathbb{M}}_{p_1 p_2 T}^*(\widehat{\theta}^{K_1 K_2})$  around  $\theta_0$  shows that

$$\begin{aligned} d^2(\widehat{\theta}^{K_1 K_2}, \theta_0) &\lesssim \bar{\mathbb{M}}_{p_1 p_2 T}^*(\widehat{\theta}^{K_1 K_2}) \\ &= \mathbb{E}[\rho_\tau(X_{ijt} - \widehat{r}_i^{K_1'} \widehat{\mathbf{F}}_t^{K_1 K_2} \widehat{c}_j^{K_2}) - \rho_\tau(X_{ijt} - r_{0i}' \mathbf{F}_{0t} c_{0j})] \leq \sup_{\theta \in \Theta^{K_1 K_2}} |\mathbb{W}_{p_1 p_2 T}(\theta)|. \end{aligned}$$

The dimension of  $r_i, \mathbf{F}_t, c_j$  does not effect the above computation process.

Secondly, it can be shown that

$$\sup_{\theta \in \Theta^{K_1 K_2}} |\mathbb{W}_{p_1 p_2 T}(\theta)| = o_p(1).$$

It derives from the linearization of  $\rho_\tau(X_{ijt} - \widehat{r}_i^{K_1'} \widehat{\mathbf{F}}_t^{K_1 K_2} \widehat{c}_j^{K_2})$  and some mathematical inequality, which are not affected by the dimension of  $r_i, \mathbf{F}_t, c_j$ .

Therefore, the proof of the above two results is similar to the proof of Lemma B.1 and it is therefore omitted.  $\square$

**Lemma C.2.** Suppose that Assumption 1 holds and  $k_1 < K_1 < \infty$ ,  $k_2 < K_2 < \infty$ . Then, for any  $\theta^{K_1 K_2} \in \Theta^{K_1 K_2}(\delta)$  and sufficiently small  $\delta$ , it holds that

$$\begin{aligned} \|\widehat{\mathbf{R}}^{K_1, k_1} - \mathbf{R}_0\|/\sqrt{p_1} &\lesssim \delta, \quad \|\widehat{\mathbf{C}}^{K_2, k_2} - \mathbf{C}_0\|/\sqrt{p_2} \lesssim \delta, \quad \|\widehat{\mathbf{F}}^{K_1 \times K_2, k_1 \times k_2} - \mathbf{F}_0\|/\sqrt{T} \lesssim \delta, \\ \|\widehat{\mathbf{F}}^{K_1 \times K_2, -(k_1 \times k_2)}\|/\sqrt{T} &\lesssim \delta, \quad \|\widehat{\mathbf{F}}^{K_1 \times K_2, k_1 \times (-k_2)}\|/\sqrt{T} \lesssim \delta, \quad \|\widehat{\mathbf{F}}^{K_1 \times K_2, (-k_1) \times k_2}\|/\sqrt{T} \lesssim \delta. \end{aligned}$$

*Proof.* The first three formulas show the distance between estimates of part of large matrix  $\mathbf{R}^{K_1}, \mathbf{F}_t^{K_1 \times K_2}, \mathbf{C}^{K_2}$  with dimension  $k_1, k_1 \times k_2, k_2$  and the true factor matrix  $\mathbf{R}_0, \mathbf{F}_{0t}, \mathbf{C}_0$ . Note the assumption of  $\mathbf{R}^{K_1}, \mathbf{F}_t^{K_1 \times K_2}, \mathbf{C}^{K_2}$ , it can be got by simple computation

$$\frac{1}{p_1} \mathbf{R}^{K_1, k_1'} \mathbf{R}^{K_1, k_1} = \mathbb{I}_{k_1}, \quad \frac{1}{p_2} \mathbf{C}^{K_2, k_2'} \mathbf{C}^{K_2, k_2} = \mathbb{I}_{k_2},$$

$$\frac{1}{T} \sum_{t=1}^T \mathbf{F}_t^{K_1 \times K_2, k_1 \times k_2} (\mathbf{F}_t^{K_1 \times K_2, k_1 \times k_2})', \quad \frac{1}{T} \sum_{t=1}^T (\mathbf{F}_t^{K_1 \times K_2, k_1 \times k_2})' \mathbf{F}_t^{K_1 \times K_2, k_1 \times k_2}$$

diagonal and descending.

Also, the definition of  $\Theta^{K_1 K_2}(\delta)$  implies that  $d(\theta^{k_1 k_2}, \theta_0) \leq \delta$ . Then, the key conditions required to prove the first three formulas are all met. The proof is similar to Lemma B.2 and it is therefore omitted.

The last three formulas show the estimates of the remaining parts of  $\mathbf{F}_t^{K_1 \times K_2}$  except the first  $k_1$  rows and  $k_2$  columns are close to zero. Since  $\widehat{\mathbf{F}}_t^{K_1 \times K_2}$  is a consistent estimator and the assumption of  $\mathbf{F}_{0t}^{K_1 \times K_2}$  for this part is set to be zero, the last three formulas thus can be obtained.  $\square$

**Lemma C.3.** *Suppose that Assumption 1 holds and  $k_1 < K_1 < \infty$ ,  $k_2 < K_2 < \infty$ . For sufficiently small  $\delta$ , it holds that*

$$\mathbb{E} \left[ \sup_{\theta^{K_1 K_2} \in \Theta^{K_1 K_2}(\delta)} |\mathbb{W}_{p_1 p_2 T}(\theta^{K_1 K_2})| \right] \lesssim \frac{\delta}{L_{p_1 p_2 T}}.$$

*Proof.* The proof applies the chaining argument which is commonly used in the theory of empirical processes and it also holds for  $K_1 > k_1$ ,  $K_2 > k_2$ . Together with Lemma C.1, Lemma C.2 and the Theorem 2.2.4 of van der Vaart and Wellner (1996), the result can be obtained.

The detail is similar to the proof of Lemma B.3 and it is therefore omitted.  $\square$

### C.3 Proof of Theorem 4.1

*Proof.* First, like in the proof of Theorem 3.2, it follows from the previous lemma that

$$d(\widehat{\theta}^{K_1 K_2}, \theta_0) = O_p(L_{p_1 p_2 T}^{-1}). \quad (30)$$

Second, similar to the proof of Lemma B.2, it can be shown that

$$|\widehat{\sigma}_{T,j}^{K_1} - \sigma_j| = o_p(1), \text{ for } j = 1, \dots, k_1. \quad |\widehat{\sigma}_{T,j}^{K_2} - \sigma'_j| = o_p(1), \text{ for } j = 1, \dots, k_2. \quad (31)$$

Third, by Lemma C.2 and (30),

$$\sum_{j=k_1+1}^{K_1} \widehat{\sigma}_{T,j}^{K_1} = \|\widehat{F}'^{K_1 \times K_2, (-k_1) \times k_2}\|^2 / T \lesssim d(\widehat{\theta}^{K_1 K_2}, \theta_0)^2 = O_p(L_{p_1 p_2 T}^{-2}). \quad (32)$$

$$\sum_{j=k_2+1}^{K_2} \widehat{\sigma}_{T,j}^{K_2} = \|\widehat{F}^{K_1 \times K_2, k_1 \times (-k_2)}\|^2 / T \lesssim d(\widehat{\theta}^{K_1 K_2}, \theta_0)^2 = O_p(L_{p_1 p_2 T}^{-2}). \quad (33)$$

Fourth, by (31)-(33), we have

$$\begin{aligned} P[\widehat{k}_1^r \neq k_1] &= P[\widehat{k}_1^r < k_1] + P[\widehat{k}_1^r > k_1] \\ &\leq P[\widehat{\sigma}_{T,k_1}^{K_1} \leq C_{p_1 p_2 T}] + P[\widehat{\sigma}_{T,k_1+1}^{K_1} > C_{p_1 p_2 T}] = o_p(1). \end{aligned} \quad (34)$$

$$\begin{aligned} P[\widehat{k}_2^r \neq k_2] &= P[\widehat{k}_2^r < k_2] + P[\widehat{k}_2^r > k_2] \\ &\leq P[\widehat{\sigma}_{T,k_2}^{K_2} \leq C_{p_1 p_2 T}] + P[\widehat{\sigma}_{T,k_2+1}^{K_2} > C_{p_1 p_2 T}] = o_p(1). \end{aligned} \quad (35)$$

Next, we prove the consistency of the rank minimization estimator set  $(\widehat{k}_1^r, \widehat{k}_2^r)$ . Let  $A = \{\widehat{k}_1^r = k_1\}$ ,  $B = \{\widehat{k}_2^r = k_2\}$ ,  $\bar{A} = \{\widehat{k}_1^r > k_1 \text{ or } \widehat{k}_1^r < k_1\}$ ,  $\bar{B} = \{\widehat{k}_2^r > k_2 \text{ or } \widehat{k}_2^r < k_2\}$ . We need to prove  $P(A \cap B) \rightarrow 1$ , which is equivalent to prove  $P(\bar{A} \cup \bar{B}) \rightarrow 0$ . According to the probability of the union and intersection of multiple events, we have

$$\begin{aligned} P(\bar{A} \cup \bar{B}) &= P(\bar{A}) + P(\bar{B}) - P(\bar{A}\bar{B}) \\ &= P(\widehat{k}_1^r > k_1 \cup \widehat{k}_1^r < k_1) + P(\widehat{k}_2^r > k_2 \cup \widehat{k}_2^r < k_2) \\ &\quad - P[(\widehat{k}_1^r > k_1 \cup \widehat{k}_1^r < k_1) \cap (\widehat{k}_2^r > k_2 \cup \widehat{k}_2^r < k_2)] \\ &= P(\widehat{k}_1^r > k_1) + P(\widehat{k}_1^r < k_1) + P(\widehat{k}_2^r > k_2) + P(\widehat{k}_2^r < k_2) \\ &\quad - P[(\widehat{k}_1^r > k_1 \cup \widehat{k}_1^r < k_1) \cap (\widehat{k}_2^r > k_2 \cup \widehat{k}_2^r < k_2)], \\ &= P(\widehat{k}_1^r > k_1) + P(\widehat{k}_1^r < k_1) + P(\widehat{k}_2^r > k_2) + P(\widehat{k}_2^r < k_2) \\ &\quad - P(\widehat{k}_1^r > k_1, \widehat{k}_2^r > k_2) - P(\widehat{k}_1^r > k_1, \widehat{k}_2^r < k_2) \\ &\quad - P(\widehat{k}_1^r < k_1, \widehat{k}_2^r > k_2) - P(\widehat{k}_1^r < k_1, \widehat{k}_2^r < k_2). \end{aligned} \quad (36)$$

Similarly, by (31)-(33), we have

$$P(\widehat{k}_1^r > k_1, \widehat{k}_2^r > k_2) \leq P(\widehat{\sigma}_{T,k_1+1}^{K_1} > C_{p_1 p_2 T}, \widehat{\sigma}_{T,k_2+1}^{K_2} > C_{p_1 p_2 T}) = o_p(1). \quad (37)$$

$$P(\widehat{k}_1^r > k_1, \widehat{k}_2^r < k_2) \leq P(\widehat{\sigma}_{T,k_1+1}^{K_1} > C_{p_1 p_2 T}, \widehat{\sigma}_{T,k_2}^{K_2} \leq C_{p_1 p_2 T}) = o_p(1). \quad (38)$$

$$P(\widehat{k}_1^r < k_1, \widehat{k}_2^r > k_2) \leq P(\widehat{\sigma}_{T,k_1}^{K_1} \leq C_{p_1 p_2 T}, \widehat{\sigma}_{T,k_2+1}^{K_2} > C_{p_1 p_2 T}) = o_p(1). \quad (39)$$

$$P(\widehat{k}_1^r < k_1, \widehat{k}_2^r < k_2) \leq P(\widehat{\sigma}_{T,k_1}^{K_1} \leq C_{p_1 p_2 T}, \widehat{\sigma}_{T,k_2}^{K_2} \leq C_{p_1 p_2 T}) = o_p(1). \quad (40)$$

Therefore, by (34)-(40), we have  $P(\bar{A} \cup \bar{B}) \rightarrow 0$ , it then shows that

$$P(A \cap B) = P(\widehat{k}_1 = k_1, \widehat{k}_2 = k_2) \rightarrow 1.$$

□

## D Proof of Theorem 4.2

Motivated by the proof in Bai and Ng (2002), it suffices to prove that:

**Case 1** for  $\ell_1 < k_1$  and  $1 \leq \ell_2 \leq K_2$ ,  $\mathbb{M}_{p_1 p_2 T}(\hat{\theta}^{\ell_1 \ell_2}) - \mathbb{M}_{p_1 p_2 T}(\hat{\theta}^{k_1 k_2}) > C + o_p(1)$  for some constant

$$C > 0,$$

**Case 2** for  $\ell_2 < k_2$  and  $1 \leq \ell_1 \leq K_1$ ,  $\mathbb{M}_{p_1 p_2 T}(\hat{\theta}^{\ell_1 \ell_2}) - \mathbb{M}_{p_1 p_2 T}(\hat{\theta}^{k_1 k_2}) > C + o_p(1)$  for some constant

$$C > 0,$$

**Case 3** for  $k_1 \leq \ell_1 \leq K_1$  and  $k_2 \leq \ell_2 \leq K_2$ ,  $\mathbb{M}_{p_1 p_2 T}(\hat{\theta}^{\ell_1 \ell_2}) - \mathbb{M}_{p_1 p_2 T}(\hat{\theta}^{k_1 k_2}) = O_p(L_{p_1 p_2 T}^{-2})$ .

Specifically, Case 1 and Case 2 are parallel, so it suffices to prove one of them. We start with Case

2. By definitions of  $\mathbb{M}$ ,  $\mathbb{M}^*$ ,  $\bar{\mathbb{M}}^*$  and  $\mathbb{W}$ , we write

$$\begin{aligned} \mathbb{M}_{p_1 p_2 T}(\hat{\theta}^{\ell_1 \ell_2}) - \mathbb{M}_{p_1 p_2 T}(\hat{\theta}^{k_1 k_2}) &= \mathbb{M}_{p_1 p_2 T}^*(\hat{\theta}^{\ell_1 \ell_2}) - \mathbb{M}_{p_1 p_2 T}^*(\hat{\theta}^{k_1 k_2}) \\ &= \bar{\mathbb{M}}_{p_1 p_2 T}^*(\hat{\theta}^{\ell_1 \ell_2}) + \mathbb{W}_{p_1 p_2 T}(\hat{\theta}^{\ell_1 \ell_2}) - \mathbb{M}_{p_1 p_2 T}^*(\hat{\theta}^{k_1 k_2}). \end{aligned}$$

Similar to the proof of (2), one can show that  $\mathbb{W}_{p_1 p_2 T}(\hat{\theta}^{\ell_1 \ell_2}) = o_p(1)$ . Further, note that  $|\rho_\tau(X_{ijt} - \hat{r}_i^{k_1'} \hat{\mathbf{F}}_t^{k_1 k_2} \hat{c}_j^{k_2}) - \rho_\tau(X_{ijt} - r'_{0i} \mathbf{F}_{0t} c_{0j})| \lesssim |\hat{r}_i^{k_1'} \hat{\mathbf{F}}_t^{k_1 k_2} \hat{c}_j^{k_2} - r'_{0i} \mathbf{F}_{0t} c_{0j}|$ . Therefore,

$$\mathbb{M}_{p_1 p_2 T}^*(\hat{\theta}^{k_1 k_2}) \lesssim d(\hat{\theta}^{k_1 k_2}, \theta_0) = o_p(1), \quad (41)$$

where the  $o_p(1)$  is by Lemma 2.1. As a result, it suffices to show that  $\bar{\mathbb{M}}_{p_1 p_2 T}^*(\hat{\theta}^{\ell_1 \ell_2}) \geq C$  for some constant  $C > 0$ .

Similar to the proof of (1) and (10), one can verify that

$$\bar{\mathbb{M}}_{p_1 p_2 T}^*(\hat{\theta}^{\ell_1 \ell_2}) \gtrsim d^2(\hat{\theta}^{\ell_1 \ell_2}, \theta_0) \gtrsim \|M_{\hat{\mathbf{C}}^{\ell_2}} \mathbf{C}_0\|^2 / p_2,$$

where  $\hat{\mathbf{C}}^{\ell_2}$  is  $p_2 \times \ell_2$  matrix constructed using the entries of  $\hat{\theta}^{\ell_1 \ell_2}$ . By definition,

$$\|M_{\hat{\mathbf{C}}^{\ell_2}} \mathbf{C}_0\|^2 / p_2 = \text{tr}(\mathbf{C}_0' \mathbf{C}_0 / p_2 - \mathbf{C}_0' \hat{\mathbf{C}}^{\ell_2} \hat{\mathbf{C}}^{\ell_2} \mathbf{C}_0 / p_2^2) = \text{tr}(\mathbb{I} - \mathbf{C}_0' \hat{\mathbf{C}}^{\ell_2} \hat{\mathbf{C}}^{\ell_2} \mathbf{C}_0 / p_2^2).$$

Note that  $\|\mathbf{C}_0' \hat{\mathbf{C}}^{\ell_2} \hat{\mathbf{C}}^{\ell_2} \mathbf{C}_0 / p_2^2\| \leq \|\mathbf{C}_0\|^2 / p_2 \times \|\hat{\mathbf{C}}^{\ell_2}\|^2 / p_2 \leq 1$ . Therefore, the eigenvalues of  $(\mathbb{I} - \mathbf{C}_0' \hat{\mathbf{C}}^{\ell_2} \hat{\mathbf{C}}^{\ell_2} \mathbf{C}_0 / p_2^2)$  are all non-negative, and we conclude that

$$\|M_{\hat{\mathbf{C}}^{\ell_2}} \mathbf{C}_0\|^2 / p_2 \geq \rho_{\max}(\mathbb{I} - \mathbf{C}_0' \hat{\mathbf{C}}^{\ell_2} \hat{\mathbf{C}}^{\ell_2} \mathbf{C}_0 / p_2^2).$$

By Lemma A.5 in Ahn and Horenstein (2013),

$$\rho_{\max}(\mathbb{I} - \mathbf{C}_0' \hat{\mathbf{C}}^{\ell_2} \hat{\mathbf{C}}^{\ell_2} \mathbf{C}_0 / p_2^2) + \rho_{\min}(\mathbf{C}_0' \hat{\mathbf{C}}^{\ell_2} \hat{\mathbf{C}}^{\ell_2} \mathbf{C}_0 / p_2^2) \geq \rho_{\min}(\mathbb{I}).$$

However,  $\mathbf{C}_0' \hat{\mathbf{C}}^{\ell_2} \hat{\mathbf{C}}^{\ell_2} \mathbf{C}_0 / p_2^2$  is a  $k_2 \times k_2$  matrix with rank equal or less than  $\ell_2 < k_2$ , which implies that  $\rho_{\min}(\mathbf{C}_0' \hat{\mathbf{C}}^{\ell_2} \hat{\mathbf{C}}^{\ell_2} \mathbf{C}_0 / p_2^2) = 0$ . Consequently, it holds that

$$\rho_{\max}(\mathbb{I} - \mathbf{C}_0' \hat{\mathbf{C}}^{\ell_2} \hat{\mathbf{C}}^{\ell_2} \mathbf{C}_0 / p_2^2) \geq 1,$$

which concludes the argument in Case 2.

It remains to consider Case 3. By definition,

$$\mathbb{M}_{p_1 p_2 T}(\hat{\theta}^{\ell_1 \ell_2}) - \mathbb{M}_{p_1 p_2 T}(\hat{\theta}^{k_1 k_2}) = \mathbb{W}_{p_1 p_2 T}(\hat{\theta}^{\ell_1 \ell_2}) - \mathbb{W}_{p_1 p_2 T}(\hat{\theta}^{k_1 k_2}) + \bar{\mathbb{M}}_{p_1 p_2 T}^*(\hat{\theta}^{\ell_1 \ell_2}) - \bar{\mathbb{M}}_{p_1 p_2 T}^*(\hat{\theta}^{k_1 k_2}).$$

For any  $k_1 \leq \ell_1 \leq K_1$  and  $k_2 \leq \ell_2 \leq K_2$ , similar to the proofs of Lemma 2.3 and Theorem 1, one can check that  $d(\hat{\theta}^{\ell_1 \ell_2}, \theta_0) = O_p(L_{p_1 p_2 T}^{-1})$  and

$$\mathbb{E} \left[ \sup_{d(\theta^{\ell_1 \ell_2}, \theta_0) \leq \delta} |\mathbb{W}_{p_1 p_2 T}(\theta^{\ell_1 \ell_2})| \right] \lesssim \frac{\delta}{L_{p_1 p_2 T}},$$

for sufficiently small  $\delta$ . Therefore, we conclude that

$$\mathbb{W}_{p_1 p_2 T}(\hat{\theta}^{\ell_1 \ell_2}) = O_p(L_{p_1 p_2 T}^{-2}), \quad k_1 \leq \ell_1 \leq K_1, k_2 \leq \ell_2 \leq K_2. \quad (42)$$

On the other hand, by a Taylor expansion and the assumption that  $|f_{ijt}(\cdot)|$  is uniformly bounded above, it can be shown that

$$|\bar{\mathbb{M}}_{p_1 p_2 T}^*(\hat{\theta}^{\ell_1 \ell_2})| \lesssim d^2(\hat{\theta}^{\ell_1 \ell_2}, \theta_0) = O_p(L_{p_1 p_2 T}^{-2}). \quad (43)$$

The formula (42) and (43) certainly hold for  $\hat{\theta}^{k_1 k_2}$ . This concludes the argument in Case 3. The consistency of  $\hat{k}_1^{IC}$  and  $\hat{k}_2^{IC}$  follows.  $\square$

## E Proof of Theorem 4.3

**Proof:** Recall the fact in Theorem 4.1,

$$|\hat{\sigma}_{T,k}^{K_1} - \sigma_k| = o_p(1), \text{ for } k = 1, \dots, k_1,$$

$$\max_{k_1+1 \leq k \leq K_1} \hat{\sigma}_{T,k}^{K_1} \leq \|\hat{F}'^{K_1 \times K_2, (-k_1) \times k_2}\|^2 / T \lesssim d(\hat{\theta}^{K_1 K_2}, \theta_0)^2 = O_p(L_{p_1 p_2 T}^{-2}).$$

It's clear that the eigenvalue ratios satisfy

$$\frac{\hat{\sigma}_{T,k}^{K_1}}{\hat{\sigma}_{T,k+1}^{K_1} + c_0 L_{p_1 p_2 T}^{-2}} \begin{cases} \asymp 1, & k \leq k_1 - 1, \\ \gtrsim L_{p_1 p_2 T}^2 \rightarrow \infty, & k = k_1, \\ \asymp 1, & k_1 + 1 \leq k \leq K_1 - 1. \end{cases}$$

That is to say, with probability tending to one, the ratio achieves maximal only at  $k = k_1$ , which implies the consistency of  $\hat{k}_1^{ER}$ . For  $\hat{k}_2^{ER}$ , the consistency can be proved in the same way and hence

omitted. It then follows that

$$P\left(\hat{k}_1^{ER} = k_1, \hat{k}_2^{ER} = k_2\right) \rightarrow 1.$$

□

## F Proof of Theorem 5.1

WE ONLY PROVE the asymptotic distribution of  $\tilde{r}_i$  since the proof for  $\tilde{c}_j$  is symmetric. Define

$\rho(u) = [\tau - K(u/h)]u$ , so that we can write the objective function as

$$\mathbb{S}_{p_1, p_2, T}(\theta) = \frac{1}{p_1 p_2 T} \sum_{i=1}^{p_1} \sum_{t=1}^T \sum_{j=1}^{p_2} \rho(X_{ijt} - r'_i F_t c_j).$$

Let  $\rho^{(s)}(u) = (\partial/\partial u)^s \rho(u)$  for  $s = 1, 2, 3$ . For fixed  $r_i, F_t, c_j$ , define

$$\bar{\rho}^{(s)}(X_{ijt} - r'_i F_t c_j) = \mathbb{E}[\rho^{(s)}(X_{ijt} - r'_i F_t c_j)],$$

$$\tilde{\rho}^{(s)}(X_{ijt} - r'_i F_t c_j) = \rho^{(s)}(X_{ijt} - r'_i F_t c_j) - \bar{\rho}^{(s)}(X_{ijt} - r'_i F_t c_j), \text{ for } s = 1, 2, 3.$$

When the functions defined above are evaluated at the true parameters, we suppress their arguments to further simplify the notations. For example,  $\rho_{ijt} = \rho(X_{ijt} - r'_{0i} F_{0t} c_{0j})$ ,  $\bar{\rho}_{ijt}^{(s)} = \bar{\rho}^{(s)}(X_{ijt} - r'_{0i} F_{0t} c_{0j})$ . Moreover, define

$$\mathbb{S}_{p_1, p_2, T}^*(\theta) = \frac{1}{p_1 p_2 T} \sum_{i=1}^{p_1} \sum_{t=1}^T \sum_{j=1}^{p_2} [\rho(X_{ijt} - r'_i F_t c_j) - \rho(X_{ijt} - r'_{0i} F_{0t} c_{0j})],$$

$$\bar{\mathbb{S}}_{p_1, p_2, T}^*(\theta) = \frac{1}{p_1 p_2 T} \sum_{i=1}^{p_1} \sum_{t=1}^T \sum_{j=1}^{p_2} \mathbb{E}[\rho(X_{ijt} - r'_i F_t c_j) - \rho(X_{ijt} - r'_{0i} F_{0t} c_{0j})],$$

$$U_{p_1, p_2, T}(\theta) = \mathbb{S}_{p_1, p_2, T}^*(\theta) - \bar{\mathbb{S}}_{p_1, p_2, T}^*(\theta).$$

Using  $\bar{O}(1)$  to denote a sequence that is uniformly (over  $i, j$  and  $t$ ) bounded. Then we can show that the following holds.

## F.1 Eight Preliminary Lemmas

**Lemma F.1.** *Under Assumptions 1 and 2, (i) There exists a constant  $\bar{C} > 0$  such that  $h^{s-1} \cdot \sup_u |\rho^s(u)| \leq \bar{C}$  for  $s = 1, 2, 3$ .*

*(ii)  $\bar{\rho}_{ijt}^{(1)} = \bar{O}(h^m)$ ,  $\bar{\rho}^{(2)}(X_{ijt} - r'_i F_t c_j) = f_{ijt}(r'_i F_t c_j - r'_{0i} F_{0t} c_{0j}) + \bar{O}(h^m)$ , and  $\bar{\rho}^{(3)}(X_{ijt} - r'_i F_t c_j) = -f_{ijt}^{(1)}(r'_i F_t c_j - r'_{0i} F_{0t} c_{0j}) + \bar{O}(h^m)$ .*

*(iii)  $\mathbb{E}(\rho_{ijt}^{(1)})^2 = \tau(1 - \tau) + \bar{O}(h)$  and  $h \cdot \mathbb{E}[(\rho_{ijt}^{(2)})^2] = \bar{O}(1)$ .*

*Proof.* Since the proof steps follow the standard ones when computing the means of kernel density estimators, they are omitted here to save space. Similar results can be found in [2] and [1].  $\square$

**Lemma F.2.** *Under Assumptions 1 and 2,  $d(\tilde{\theta}, \theta_0) = o_p(1)$  as  $p_1, p_2, T \rightarrow \infty$  and  $h \rightarrow 0$ .*

*Proof.* By definition, we have  $\mathbb{S}_{p_1 p_2 T}(\tilde{\theta}) \leq \mathbb{S}_{p_1 p_2 T}(\theta_0)$ . Adding and subtracting terms, we have

$$d^2(\tilde{\theta}, \theta_0) \leq \bar{\mathbb{M}}_{p_1 p_2 T}^*(\tilde{\theta}) \leq \mathbb{M}_{p_1 p_2 T}(\tilde{\theta}) - \mathbb{S}_{p_1 p_2 T}(\tilde{\theta}) + \mathbb{S}_{p_1 p_2 T}(\theta_0) - \mathbb{M}_{p_1 p_2 T}(\theta_0) - \mathbb{W}_{p_1 p_2 T}(\tilde{\theta}).$$

It follows that

$$d^2(\tilde{\theta}, \theta_0) \leq \sup_{\theta \in \Theta^{k_1 k_2}} |\mathbb{M}_{p_1 p_2 T}(\theta) - \mathbb{S}_{p_1 p_2 T}(\theta)| + \sup_{\theta \in \Theta^{k_1 k_2}} |\mathbb{W}_{p_1 p_2 T}(\theta)|.$$

It is easy to see that the first term on the RHS of the above inequality is  $O_p(h)$ , and the second term is  $o_p(1)$  as proved in Lemma B.1. Then, the desired result follows.  $\square$

**Lemma F.3.** *Under Assumptions 1 and 2,  $d(\tilde{\theta}, \theta_0) = O_p(1/L_{p_1 p_2 T})$  as  $p_1, p_2, T \rightarrow \infty$ .*

*Proof.* First, since  $\rho^{(1)}(u)$  is uniformly bounded, we have  $|\rho(X_{ijt} - c_1) - \rho(X_{ijt} - c_2)| \lesssim |c_1 - c_2|$ .

Then similar to the proof of Lemma B.3, we can show that

$$\mathbb{E} \left[ \sup_{\theta \in \Theta^{k_1 k_2}(\delta)} |U_{p_1 p_2 T}(\theta)| \right] \lesssim \frac{\delta}{L_{p_1 p_2 T}}. \quad (44)$$

Analogous to the proof of Theorem 1, the parameter space  $\Theta^{k_1 k_2}$  can be partitioned into shells  $S_j = \{\theta \in \Theta^{k_1 k_2} : 2^{j-1} < L_{p_1 p_2 T} \cdot d(\theta, \theta_0) \leq 2^j\}$ . Conclude that, for a given integer  $V$  and for every

$\eta > 0$ ,

$$P[L_{p_1 p_2 T} \cdot d(\tilde{\theta}, \theta_0) > 2^V] \leq \sum_{j > V, 2^{j-1} \leq \eta L_{p_1 p_2 T}} P\left[\inf_{\theta \in S_j} \mathbb{S}_{p_1 p_2 T}^*(\theta) \leq 0\right] + P[d(\tilde{\theta}, \theta_0) > \eta].$$

For arbitrarily small  $\eta > 0$ , the second probability on the RHS of the above equation converges to 0 as  $p_1, p_2, T \rightarrow \infty$  by Lemma F.2.

Next, expanding  $\mathbb{S}_{p_1 p_2 T}^*(\theta)$  around  $\theta_0$  and taking expectations yield

$$\bar{\mathbb{S}}_{p_1 p_2 T}^*(\theta) = \frac{1}{T p_1 p_2} \sum_{i=1}^{p_1} \sum_{t=1}^T \sum_{j=1}^{p_2} \bar{\rho}_{ijt}^{(1)} \cdot (r'_i F_t c_j - r'_{0i} F_{0t} c_{0j}) + \frac{1}{T p_1 p_2} \sum_{i=1}^{p_1} \sum_{t=1}^T \sum_{j=1}^{p_2} 0.5 \bar{\rho}^{(2)}(c_{ijt}^*) \cdot (r'_i F_t c_j - r'_{0i} F_{0t} c_{0j})^2,$$

where  $c_{ijt}^*$  lies between  $r'_i F_t c_j$  and  $r'_{0i} F_{0t} c_{0j}$ . It then follows from Lemma F.1 and Assumption 2 that

$$\bar{\mathbb{S}}_{p_1 p_2 T}^*(\theta) \geq O(h^m) + 0.5 \underline{f} \cdot d^2(\theta, \theta_0).$$

Thus, for each  $\theta$  in  $S_j$  we have

$$-\bar{\mathbb{S}}_{p_1 p_2 T}^*(\theta) \leq -0.5 \underline{f} \cdot d^2(\theta, \theta_0) + O(h^m) \leq -\underline{f} \cdot \frac{2^{2j-3}}{L_{p_1 p_2 T}^2} + O(h^m).$$

Therefore,  $\inf_{\theta \in S_j} \mathbb{S}_{p_1 p_2 T}^*(\theta) \leq 0$  implies that

$$\inf_{\theta \in S_j} \mathbb{U}_{p_1 p_2 T}(\theta) \leq -\underline{f} \cdot \frac{2^{2j-3}}{L_{p_1 p_2 T}^2} + O(h^m),$$

and it follows that

$$\sum_{j > V, 2^{j-1} \leq \eta L_{p_1 p_2 T}} P\left[\inf_{\theta \in S_j} \mathbb{S}_{p_1 p_2 T}^*(\theta) \leq 0\right] \leq \sum_{j > V, 2^{j-1} \leq \eta L_{p_1 p_2 T}} P\left[\sup_{\theta \in S_j} |\mathbb{U}_{p_1 p_2 T}(\theta)| \geq \underline{f} \cdot \frac{2^{2j-3}}{L_{p_1 p_2 T}^2} + O(h^m)\right].$$

By (44) and Markov's inequality, we have

$$P\left[\sup_{\theta \in S_j} |\mathbb{U}_{p_1 p_2 T}(\theta)| \geq \underline{f} \cdot \frac{2^{2j-3}}{L_{p_1 p_2 T}^2} + O(h^m)\right] \lesssim \frac{2^j}{2^{2j} + O(L_{p_1 p_2 T}^2 \cdot h^m)}.$$

By Assumption 2(v),  $O(L_{p_1 p_2 T}^2 \cdot h^m) = o(1)$ . Thus, the above inequality implies that

$$\sum_{j > V, 2^{j-1} \leq \eta L_{p_1 p_2 T}} P\left[\inf_{\theta \in S_j} \mathbb{S}_{p_1 p_2 T}^*(\theta) \leq 0\right] \lesssim \sum_{j > V} 2^{-j}.$$

The RHS of the previous expression converges to 0 as  $V \rightarrow \infty$ , implying that  $L_{p_1 p_2 T} \cdot d(\tilde{\theta}, \theta) = O_p(1)$ ,

or  $d(\tilde{\theta}, \theta) = O_p(1/L_{p_1 p_2 T})$ .  $\square$

Define:

$$\begin{aligned}
\mathbb{S}_{i,T,p_2}^*(r, F, c) &= \frac{1}{Tp_2} \sum_{t=1}^T \sum_{j=1}^{p_2} [\rho(X_{ijt} - r'F_t c_j) - \rho(X_{ijt} - r'_{0i} F_{0t} c_{0j})], \\
\bar{\mathbb{S}}_{i,T,p_2}^*(r, F, c) &= \frac{1}{Tp_2} \sum_{t=1}^T \sum_{j=1}^{p_2} \mathbb{E}[\rho(X_{ijt} - r'F_t c_j) - \rho(X_{ijt} - r'_{0i} F_{0t} c_{0j})], \\
\mathbb{M}_{i,T,p_2}^*(r, F, c) &= \frac{1}{Tp_2} \sum_{t=1}^T \sum_{j=1}^{p_2} [\rho_\tau(X_{ijt} - r'F_t c_j) - \rho_\tau(X_{ijt} - r'_{0i} F_{0t} c_{0j})], \\
\bar{\mathbb{M}}_{i,T,p_2}^*(r, F, c) &= \frac{1}{Tp_2} \sum_{t=1}^T \sum_{j=1}^{p_2} \mathbb{E}[\rho_\tau(X_{ijt} - r'F_t c_j) - \rho_\tau(X_{ijt} - r'_{0i} F_{0t} c_{0j})].
\end{aligned}$$

**Lemma F.4.** *Under Assumptions 1 and 2, we have  $\|\tilde{r}_i - r_{0i}\| = o_p(1)$  for each  $i$ .*

*Proof.* Note that

$$\tilde{r}_i = \arg \min_{r \in \mathcal{A}} \mathbb{S}_{i,T,p_2}^*(r, \tilde{F}, \tilde{c}).$$

First, we show that

$$\sup_{r \in \mathcal{A}} |\mathbb{S}_{i,T,p_2}^*(r, \tilde{F}, \tilde{c}) - \bar{\mathbb{M}}_{i,T,p_2}^*(r, F_0, c_0)| = o_p(1). \quad (45)$$

Adding and subtracting terms, we have

$$\begin{aligned}
&\mathbb{S}_{i,T,p_2}^*(r, \tilde{F}, \tilde{c}) - \bar{\mathbb{M}}_{i,T,p_2}^*(r, F_0, c_0) \\
&= \mathbb{S}_{i,T,p_2}^*(r, \tilde{F}, \tilde{c}) - \mathbb{M}_{i,T,p_2}^*(r, \tilde{F}, \tilde{c}) + \mathbb{M}_{i,T,p_2}^*(r, \tilde{F}, \tilde{c}) - \mathbb{M}_{i,T,p_2}^*(r, F_0, \tilde{c}) \\
&\quad + \mathbb{M}_{i,T,p_2}^*(r, F_0, \tilde{c}) - \mathbb{M}_{i,T,p_2}^*(r, F_0, c_0) + \mathbb{M}_{i,T,p_2}^*(r, F_0, c_0) - \bar{\mathbb{M}}_{i,T,p_2}^*(r, F_0, c_0).
\end{aligned}$$

thus,

$$\begin{aligned}
&\sup_{r \in \mathcal{A}} |\mathbb{S}_{i,T,p_2}^*(r, \tilde{F}, \tilde{c}) - \bar{\mathbb{M}}_{i,T,p_2}^*(r, F_0, c_0)| \\
&\leq \sup_{r \in \mathcal{A}} |\mathbb{S}_{i,T,p_2}^*(r, \tilde{F}, \tilde{c}) - \mathbb{M}_{i,T,p_2}^*(r, \tilde{F}, \tilde{c})| + \sup_{r \in \mathcal{A}} |\mathbb{M}_{i,T,p_2}^*(r, \tilde{F}, \tilde{c}) - \mathbb{M}_{i,T,p_2}^*(r, F_0, \tilde{c})| \\
&\quad + \sup_{r \in \mathcal{A}} |\mathbb{M}_{i,T,p_2}^*(r, F_0, \tilde{c}) - \mathbb{M}_{i,T,p_2}^*(r, F_0, c_0)| + \sup_{r \in \mathcal{A}} |\mathbb{M}_{i,T,p_2}^*(r, F_0, c_0) - \bar{\mathbb{M}}_{i,T,p_2}^*(r, F_0, c_0)|.
\end{aligned}$$

It is easy to show that

$$\begin{aligned}
\sup_{r \in \mathcal{A}} |\mathbb{S}_{i,T,p_2}^*(r, \tilde{F}, \tilde{c}) - \mathbb{M}_{i,T,p_2}^*(r, \tilde{F}, \tilde{c})| &\lesssim h, \\
\sup_{r \in \mathcal{A}} |\mathbb{M}_{i,T,p_2}^*(r, \tilde{F}, \tilde{c}) - \mathbb{M}_{i,T,p_2}^*(r, F_0, \tilde{c})| &\lesssim \sup_{r \in \mathcal{A}} \|r\| \cdot \|\tilde{c}\| \cdot \frac{1}{T} \sum_{t=1}^T \|\tilde{F}_t - F_{0t}\| \\
&\lesssim \|\tilde{F} - F_0\|/\sqrt{T} = O_p(1/L_{p_1 p_2 T}), \\
\sup_{r \in \mathcal{A}} |\mathbb{M}_{i,T,p_2}^*(r, F_0, \tilde{c}) - \mathbb{M}_{i,T,p_2}^*(r, F_0, c_0)| &\lesssim \sup_{r \in \mathcal{A}} \|r\| \cdot \|F_0\| \cdot \frac{1}{p_2} \sum_{j=1}^{p_2} \|\tilde{c}_j - c_{0j}\| \\
&\lesssim \|\tilde{C} - C_0\|/\sqrt{p_2} = O_p(1/L_{p_1 p_2 T}), \\
\sup_{r \in \mathcal{A}} |\mathbb{M}_{i,T,p_2}^*(r, F_0, c_0) - \bar{\mathbb{M}}_{i,T,p_2}^*(r, F_0, c_0)| &= o_p(1).
\end{aligned}$$

Then (45) follows as  $h \rightarrow 0$ .

Second, we can show that for any  $\epsilon > 0$ , and  $B_i(\epsilon) = \{r \in \mathcal{A} : \|r - r_{0i}\| \leq \epsilon\}$ ,

$$\inf_{r \in B_i^C(\epsilon)} \bar{\mathbb{M}}_{i,T,p_2}^*(r, F_0, c_0) > \bar{\mathbb{M}}_{i,T,p_2}^*(r_{0i}, F_0, c_0) = 0, \tag{46}$$

for example, the proof of Proposition 3.1 of [1].

Finally, given (45) and (46), the consistency of  $\tilde{r}_i$  follows from a standard consistency proof of M-estimators (see Theorem 2.1 of [3]), so that the proof concludes.  $\square$

**Lemma F.5.** *Under Assumptions 1 and 2, we have  $\|\tilde{r}_i - r_{0i}\| = O_p((Tp_2)^{-\frac{1}{2}}h^{-1})$  for each  $i$ .*

*Proof.* For any fixed  $r_i \in \mathcal{A}$ ,  $F_t \in \mathcal{F}$  and  $c_j \in \mathcal{B}$ , expanding  $\rho^{(1)}(X_{ijt} - r'_i F_t c_j) F_t c_j$  gives

$$\begin{aligned}
& \rho^{(1)}(X_{ijt} - r'_i F_t c_j) F_t c_j \\
&= \rho^{(1)}(X_{ijt} - r'_{0i} F_t c_j) F_t c_j - \rho^{(2)}(X_{ijt} - r'_{0i} F_t c_j) F_t c_j c'_j F'_t (r_i - r_{0i}) \\
&+ 0.5 \rho^{(3)}(X_{ijt} - r'^*_i F_t c_j) F_t c_j [(r_i - r_{0i})' F_t c_j]^2 \\
&= \rho^{(1)}_{ijt} F_{0t} c_{0j} + \rho^{(1)}(X_{ijt} - r'_{0i} F_t^* c_j^*)(F_t c_j - F_{0t} c_{0j}) - \rho^{(2)}(X_{ijt} - r'_{0i} F_t^* c_j^*) F_t^* c_j^* r'_{0i} (F_t c_j - F_{0t} c_{0j}) \\
&- \rho^{(2)}_{ijt} F_t c_j c'_j F'_t (r_i - r_{0i}) + \rho^{(3)}(X_{ijt} - r'_{0i} F_t^* c_j^*) F_t c_j c'_j F'_t (r_i - r_{0i}) r'_{0i} (F_t c_j - F_{0t} c_{0j}) \\
&+ 0.5 \rho^{(3)}(X_{ijt} - r'^*_i F_t c_j) F_t c_j [(r_i - r_{0i})' F_t c_j]^2 \\
&= \rho^{(1)}_{ijt} F_{0t} c_{0j} + \rho^{(1)}(X_{ijt} - r'_{0i} F_t^* c_j^*)(F_t - F_{0t}) c_j + \rho^{(1)}(X_{ijt} - r'_{0i} F_t^* c_j^*) F_{0t} (c_j - c_{0j}) \\
&- \rho^{(2)}(X_{ijt} - r'_{0i} F_t^* c_j^*) F_t^* c_j^* r'_{0i} (F_t - F_{0t}) c_j - \rho^{(2)}(X_{ijt} - r'_{0i} F_t^* c_j^*) F_t^* c_j^* r'_{0i} F_{0t} (c_j - c_{0j}) \\
&- \rho^{(2)}_{ijt} F_t c_j c'_j F'_t (r_i - r_{0i}) + \rho^{(3)}(X_{ijt} - r'_{0i} F_t^* c_j^*) F_t c_j c'_j F'_t (r_i - r_{0i}) r'_{0i} (F_t - F_{0t}) c_j \\
&+ \rho^{(3)}(X_{ijt} - r'_{0i} F_t^* c_j^*) F_t c_j c'_j F'_t (r_i - r_{0i}) r'_{0i} F_{0t} (c_j - c_{0j}) + 0.5 \rho^{(3)}(X_{ijt} - r'^*_i F_t c_j) F_t c_j [(r_i - r_{0i})' F_t c_j]^2,
\end{aligned}$$

where  $r_i^*$  lies between  $r_i$  and  $r_{0i}$ ,  $F_t^*$  lies between  $F_t$  and  $F_{0t}$ ,  $c_j^*$  lies between  $c_j$  and  $c_{0j}$ . Taking expectations of both sides of the above equation, and setting  $r_i = \tilde{r}_i$ ,  $F_t = \tilde{F}_t$ ,  $c_j = \tilde{c}_j$ , it follows

from Lemma C.2 that

$$\begin{aligned}
& \frac{1}{Tp_2} \sum_{t=1}^T \sum_{j=1}^{p_2} \bar{\rho}^{(1)}(X_{ijt} - \tilde{r}'_i \tilde{F}_t \tilde{c}_j) \tilde{F}_t \tilde{c}_j \\
&= \frac{1}{Tp_2} \sum_{t=1}^T \sum_{j=1}^{p_2} \bar{\rho}^{(1)}_{ijt} F_{0t} c_{0j} - \frac{1}{Tp_2} \sum_{t=1}^T \sum_{j=1}^{p_2} \bar{\rho}^{(2)}_{ijt} \tilde{F}_t \tilde{c}_j \tilde{c}'_j \tilde{F}'_t (\tilde{r}_i - r_{0i}) \\
&+ O_p(\|\tilde{r}'_i - r_{0i}\|) \cdot O_p(T^{-1/2} \|\tilde{F} - F_0\|) + O_p(T^{-1/2} \|\tilde{F} - F_0\|) + O_p(p_2^{-1/2} \|\tilde{C} - C_0\|) \\
&+ O_p(\|\tilde{r}'_i - r_{0i}\|) \cdot O_p(p_2^{-1/2} \|\tilde{C} - C_0\|) + O_p(\|\tilde{r}'_i - r_{0i}\|^2).
\end{aligned}$$

Lemma F.1, Lemma F.3, and Assumption 2 imply that

$$\frac{1}{Tp_2} \sum_{t=1}^T \sum_{j=1}^{p_2} \bar{\rho}^{(2)}_{ijt} \tilde{F}_t \tilde{c}_j \tilde{c}'_j \tilde{F}'_t = \frac{1}{Tp_2} \sum_{t=1}^T \sum_{j=1}^{p_2} \bar{\rho}^{(2)}_{ijt} F_{0t} c_{0j} c'_{0j} F'_{0t} + o_p(1) = \Phi_i + o_p(1).$$

Then, from Lemmas F.1, F.3, and F.4, we get

$$\Phi_i(\tilde{r}_i - r_{0i}) + o_p(\|\tilde{r}_i - r_{0i}\|) = O(h^m) + O_p(1/L_{p_1 p_2 T}) - \frac{1}{Tp_2} \sum_{t=1}^T \sum_{j=1}^{p_2} \bar{\rho}^{(1)}(X_{ijt} - \tilde{r}'_i \tilde{F}_t \tilde{c}_j) \tilde{F}_t \tilde{c}_j. \quad (47)$$

Note that we can write

$$\begin{aligned}
& \frac{1}{Tp_2} \sum_{t=1}^T \sum_{j=1}^{p_2} \bar{\rho}^{(1)}(X_{ijt} - \tilde{r}'_i \tilde{F}_t \tilde{c}_j) \tilde{F}_t \tilde{c}_j \\
&= \frac{1}{Tp_2} \sum_{t=1}^T \sum_{j=1}^{p_2} \tilde{\rho}_{ijt}^{(1)} F_{0t} c_{0j} - \frac{1}{Tp_2} \sum_{t=1}^T \sum_{j=1}^{p_2} [\tilde{\rho}^{(1)}(X_{ijt} - \tilde{r}'_i \tilde{F}_t \tilde{c}_j) \tilde{F}_t \tilde{c}_j - \tilde{\rho}_{ijt}^{(1)} F_{0t} c_{0j}] \\
&= -\frac{1}{Tp_2} \sum_{t=1}^T \sum_{j=1}^{p_2} \tilde{\rho}_{ijt}^{(1)} F_{0t} c_{0j} - \frac{1}{Tp_2} \sum_{t=1}^T \sum_{j=1}^{p_2} [\tilde{\rho}^{(1)}(X_{ijt} - \tilde{r}'_i \tilde{F}_t \tilde{c}_j) \tilde{F}_t \tilde{c}_j - \tilde{\rho}^{(1)}(X_{ijt} - \tilde{r}'_i F_{0t} c_{0j}) F_{0t} c_{0j}] \\
&\quad - \frac{1}{Tp_2} \sum_{t=1}^T \sum_{j=1}^{p_2} [\tilde{\rho}^{(1)}(X_{ijt} - \tilde{r}'_i F_{0t} c_{0j}) - \tilde{\rho}_{ijt}^{(1)}] F_{0t} c_{0j}.
\end{aligned}$$

The first term on the RHS of the above equation is  $O_p((Tp_2)^{-1/2})$  by Lemma F.1 and Lyapunov's CLT. As for the second term on the RHS of the above equation, we have that

$$\begin{aligned}
& \frac{1}{Tp_2} \sum_{t=1}^T \sum_{j=1}^{p_2} [\tilde{\rho}^{(1)}(X_{ijt} - \tilde{r}'_i \tilde{F}_t \tilde{c}_j) \tilde{F}_t \tilde{c}_j - \tilde{\rho}^{(1)}(X_{ijt} - \tilde{r}'_i F_{0t} c_{0j}) F_{0t} c_{0j}] \\
&= \frac{1}{Tp_2} \sum_{t=1}^T \sum_{j=1}^{p_2} \tilde{\rho}^{(1)}(X_{ijt} - \tilde{r}'_i F_t^* c_j^*) (\tilde{F}_t - F_{0t}) \tilde{c}_j + \frac{1}{Tp_2} \sum_{t=1}^T \sum_{j=1}^{p_2} \tilde{\rho}^{(1)}(X_{ijt} - \tilde{r}'_i F_t^* c_j^*) F_{0t} (\tilde{c}_j - c_{0j}) \\
&\quad - \frac{1}{Tp_2} \sum_{t=1}^T \sum_{j=1}^{p_2} \tilde{\rho}^{(2)}(X_{ijt} - \tilde{r}'_i F_t^* c_j^*) F_t^* c_j^* \tilde{r}'_i (\tilde{F}_t - F_{0t}) \tilde{c}_j \\
&\quad - \frac{1}{Tp_2} \sum_{t=1}^T \sum_{j=1}^{p_2} \tilde{\rho}^{(2)}(X_{ijt} - \tilde{r}'_i F_t^* c_j^*) F_t^* c_j^* F_{0t} (\tilde{c}_j - c_{0j}). \tag{48}
\end{aligned}$$

where  $F_t^*$  lies between  $\tilde{F}_t$  and  $F_{0t}$ ,  $c_j^*$  lies between  $\tilde{c}_j$  and  $c_{0j}$ . The first and second terms on the RHS of (48) are  $O_p(1/L_{p_1 p_2 T})$  because  $\rho^{(1)}$  is uniformly bounded and  $\frac{1}{T} \sum_{t=1}^T \|\tilde{F}_t - F_{0t}\| = O_p(1/L_{p_1 p_2 T})$ ,  $\frac{1}{p_2} \sum_{j=1}^{p_2} \|\tilde{c}_j - c_{0j}\| = O_p(1/L_{p_1 p_2 T})$  by Lemma F.3. Similarly, the second term on the RHS of (48) is  $O_p(1/L_{p_1 p_2 T} h)$  because  $h\rho^{(2)}(u)$  is uniformly bounded. Finally, we can show that (see, e.g., Lemma B.2 of [1])

$$\frac{1}{Tp_2} \sum_{t=1}^T \sum_{j=1}^{p_2} [\tilde{\rho}^{(1)}(X_{ijt} - \tilde{r}'_i F_{0t} c_{0j}) - \tilde{\rho}_{ijt}^{(1)}] F_{0t} c_{0j} = O_p(\|\tilde{r}_i - r_{0i}\|) \cdot O_p(1/\sqrt{Tp_2 h}) = o_p(\|\tilde{r}_i - r_{0i}\|).$$

Combining the above results yields

$$\frac{1}{Tp_2} \sum_{t=1}^T \sum_{j=1}^{p_2} \bar{\rho}^{(1)}(X_{ijt} - \tilde{r}'_i \tilde{F}_t \tilde{c}_j) \tilde{F}_t \tilde{c}_j = O_p((Tp_2)^{-\frac{1}{2}}) + O_p(1/L_{p_1 p_2 T}) + O_p(1/L_{p_1 p_2 T} h) + o_p(\|\tilde{r}_i - r_{0i}\|), \tag{49}$$

and the desired result follows from (47), (49), and Assumption 2.  $\square$

To derive the asymptotic distribution of  $\tilde{r}_i$ , it is essential to obtain the stochastic expansion of  $\tilde{F}_t$  and  $\tilde{c}_j$ . To do so, define

$$\begin{aligned} \mathbb{P}_{p_1 p_2 T}(\theta) = & b \left[ \frac{1}{2p_1} \sum_{p=1}^{k_1} \sum_{q>p}^{k_1} \left( \sum_{i=1}^{p_1} r_{ip} r_{iq} \right)^2 + \frac{1}{2Tp_2} \sum_{p=1}^{k_1} \sum_{q>p}^{k_1} \left( \sum_{t=1}^T \sum_{j=1}^{p_2} (F_t c_j)_p (F_t c_j)_q \right)^2 \right. \\ & \left. + \frac{1}{8Tp_2} \sum_{p=1}^{k_1} \left( \sum_{t=1}^T \sum_{j=1}^{p_2} (F_t c_j)_p^2 - T \right)^2 \right] \end{aligned}$$

for some  $b > 0$ . Define

$$\begin{aligned} S^*(\theta) = & \left[ \dots, -\frac{1}{\sqrt{p_1 p_2 T}} \sum_{t=1}^T \sum_{j=1}^{p_2} \bar{\rho}^{(1)}(X_{ijt} - r'_i F_t c_j) F_t c_j, \dots, \dots, -\frac{1}{\sqrt{p_1 p_2 T}} \sum_{t=1}^T \sum_{j=1}^{p_2} \bar{\rho}^{(1)}(X_{ijt} - r'_i F_t c_j) r_i c'_j, \right. \\ & \left. \dots, \dots, -\frac{1}{\sqrt{p_1 p_2 T}} \sum_{t=1}^T \sum_{j=1}^{p_2} \bar{\rho}^{(1)}(X_{ijt} - r'_i F_t c_j) F'_t r_i, \dots \right], \end{aligned}$$

$$S(\theta) = S^*(\theta) + \partial \mathbb{P}_{p_1 p_2 T}(\theta) / \partial \theta, \quad \mathcal{H} = \partial S^*(\theta) / \partial \theta' + \partial^2 \mathbb{P}_{p_1 p_2 T}(\theta) / \partial \theta \partial \theta',$$

and let  $\mathcal{H} = \mathcal{H}(\theta_0)$ .

Expanding  $S(\tilde{\theta})$  around  $S(\theta_0)$  gives

$$S(\tilde{\theta}) = S(\theta_0) + \mathcal{H} \cdot (\tilde{\theta} - \theta_0) + 0.5 \mathcal{R}(\tilde{\theta}), \quad (50)$$

where

$$\mathcal{R}(\tilde{\theta}) = \left( \sum_{j=1}^M \partial \mathcal{H}(\theta^*) / \partial \theta_j \cdot (\tilde{\theta}_j - \theta_{0j}) \right) (\tilde{\theta} - \theta_0),$$

and  $\theta^*$  lies between  $\tilde{\theta}$  and  $\theta_0$ .

Further, define

$$\mathcal{H}_d = \begin{pmatrix} \mathcal{H}_d^R & \mathbf{0} & \mathbf{0} \\ \mathbf{0} & \mathcal{H}_d^F & \mathbf{0} \\ \mathbf{0} & \mathbf{0} & \mathcal{H}_d^C \end{pmatrix}, \quad \mathcal{H}_d^R = \frac{\sqrt{T p_2}}{\sqrt{p_1}} \text{diag}[\Phi_{Tp_2,1}, \dots, \Phi_{Tp_2,i}, \dots, \Phi_{Tp_2,p_1}],$$

$$\mathcal{H}_d^F = \frac{\sqrt{p_1 p_2}}{\sqrt{T}} \text{diag}[\Psi_{p_1 p_2,1}, \dots, \Psi_{p_1 p_2,t}, \dots, \Psi_{p_1 p_2,T}], \quad \mathcal{H}_d^C = \frac{\sqrt{T p_1}}{\sqrt{p_2}} \text{diag}[\varphi_{Tp_1,1}, \dots, \varphi_{Tp_1,j}, \dots, \varphi_{Tp_1,p_2}],$$

where

$$\begin{aligned}\Phi_{Tp_2,i} &= \frac{1}{Tp_2} \sum_{t=1}^T \sum_{j=1}^{p_2} \bar{\rho}_{ijt}^{(2)} F_{0t} c_{0j} c'_{0j} F'_{0t}, \quad \Psi_{p_1 p_2, t} = \frac{1}{p_1 p_2} \sum_{i=1}^{p_1} \sum_{j=1}^{p_2} \bar{\rho}_{ijt}^{(2)} (r_{0i} c'_{0j})^2, \\ \varphi_{Tp_1,j} &= \frac{1}{Tp_1} \sum_{t=1}^T \sum_{i=1}^{p_1} \bar{\rho}_{ijt}^{(2)} F'_{0t} r_{0i} r'_{0i} F_{0t}.\end{aligned}$$

The following lemma is important for the stochastic expansion of  $\tilde{F}_t$  and  $\tilde{c}_j$ .

**Lemma F.6.** *The matrix  $\mathcal{H}$  is invertible and  $\|\mathcal{H}^{-1} - \mathcal{H}_d^{-1}\|_{\max} = O(1/Tp_2)$ .*

*Proof.* To simplify the notations, we consider the case  $k_1 = k_2 = 2$ , but the proof can be easily generalized to the case  $k_1 > 2, k_2 > 2$ . Note that  $r_{0i} = (r_{0i,1}, r_{0i,2})'$ ,  $F_{0t} = (F_{0t,11}, F_{0t,12}; F_{0t,21}, F_{0t,22})$  and  $c_{0j} = (c_{0j,1}, c_{0j,2})'$ , and  $P_{p_1 p_2 T}(\theta)$  simplifies to

$$\begin{aligned}\mathbb{P}_{p_1 p_2 T}(\theta) &= b \left[ \frac{1}{2p_1} \left( \sum_{i=1}^{p_1} r_{i1} r_{i2} \right)^2 + \frac{1}{2Tp_2} \left( \sum_{t=1}^T \sum_{j=1}^{p_2} (F_t c_j)_1 (F_t c_j)_2 \right)^2 \right. \\ &\quad \left. + \frac{1}{8Tp_2} \sum_{p=1}^{k_1} \left( \sum_{t=1}^T \sum_{j=1}^{p_2} (F_t c_j)_1^2 - T \right)^2 + \frac{1}{8Tp_2} \sum_{p=1}^{k_1} \left( \sum_{t=1}^T \sum_{j=1}^{p_2} (F_t c_j)_2^2 - T \right)^2 \right]\end{aligned}$$

First, define

$$\begin{aligned}\gamma'_1 &= \left[ \mathbf{0}_{1 \times 2p_1}, ((F_{01} c_{01})_1, 0), \dots, ((F_{0t} c_{0j})_1, 0), \dots, ((F_T c_{p_2})_1, 0) \right] / \sqrt{Tp_2}, \\ \gamma'_2 &= \left[ \mathbf{0}_{1 \times 2p_1}, (0, (F_{01} c_{01})_2), \dots, (0, (F_{0t} c_{0j})_2), \dots, (0, (F_T c_{p_2})_2) \right] / \sqrt{Tp_2}, \\ \gamma'_3 &= \left[ \mathbf{0}_{1 \times 2p_1}, ((F_{01} c_{01})_2, (F_{01} c_{01})_1), \dots, ((F_{0t} c_{0j})_2, (F_{0t} c_{0j})_1), \dots, ((F_T c_{p_2})_2, (F_T c_{p_2})_1) \right] / \sqrt{Tp_2}, \\ \gamma'_4 &= \left[ (r_{01,2}, r_{01,1}), \dots, (r_{0i,2}, r_{0i,1}), \dots, (r_{0p_1,2}, r_{0p_1,1}), \mathbf{0}_{1 \times 2Tp_2} \right] / \sqrt{p_1},\end{aligned}$$

and note that  $\partial^2 \mathbb{P}_{p_1 p_2 T}(\theta_0) / \partial \theta \partial \theta' = b(\sum_{k=1}^4 \gamma_k \gamma'_k)$ .

Second, define

$$\begin{aligned}
& w'_1 \\
& = [\underbrace{(F'_{01}r_{01,1}, 0)/\sqrt{Tp_1}, \dots, (F'_{0T}c_{0p_1,1}, 0)/\sqrt{Tp_1}}_{w'_{1R}}, \underbrace{(r_{01}c'_{01,1}, \mathbf{0}_{1 \times 2})/\sqrt{p_1p_2}, \dots, (r_{0p_1}c'_{0p_2,1}, \mathbf{0}_{1 \times 2})/\sqrt{p_1p_2}}_{w'_{1F}}, \\
& \quad \underbrace{(F_{01}c_{01,1}, 0)/\sqrt{Tp_2}, \dots, (F_{0T}c_{0p_2,1}, 0)/\sqrt{Tp_2}}_{w'_{1C}}], \\
& w'_2 \\
& = [\underbrace{(0, F'_{01}r_{01,2})/\sqrt{Tp_1}, \dots, (0, F'_{0T}c_{0p_1,2})/\sqrt{Tp_1}}_{w'_{2R}}, \underbrace{(\mathbf{0}_{1 \times 2}, r_{01}c'_{01,2})/\sqrt{p_1p_2}, \dots, (\mathbf{0}_{1 \times 2}, r_{0p_1}c'_{0p_2,2})/\sqrt{p_1p_2}}_{w'_{2F}}, \\
& \quad \underbrace{(0, F_{01}c_{01,2})/\sqrt{Tp_2}, \dots, (0, F_{0T}c_{0p_2,2})/\sqrt{Tp_2}}_{w'_{2C}}], \\
& w'_3 \\
& = [\underbrace{(0, F'_{01}r_{01,1})/\sqrt{Tp_1}, \dots, (0, F'_{0T}c_{0p_1,1})/\sqrt{Tp_1}}_{w'_{3R}}, \underbrace{(\mathbf{0}_{1 \times 2}, r_{01}c'_{01,1})/\sqrt{p_1p_2}, \dots, (\mathbf{0}_{1 \times 2}, r_{0p_1}c'_{0p_2,1})/\sqrt{p_1p_2}}_{w'_{3F}}, \\
& \quad \underbrace{(F_{01}c_{01,2}, 0)/\sqrt{Tp_2}, \dots, (F_{0T}c_{0p_2,2}, 0)/\sqrt{Tp_2}}_{w'_{3C}}], \\
& w'_4 \\
& = [\underbrace{(F'_{01}r_{01,2}, 0)/\sqrt{Tp_1}, \dots, (F'_{0T}c_{0p_1,2}, 0)/\sqrt{Tp_1}}_{w'_{4R}}, \underbrace{(r_{01}c'_{01,2}, \mathbf{0}_{1 \times 2})/\sqrt{p_1p_2}, \dots, (r_{0p_1}c'_{0p_2,2}, \mathbf{0}_{1 \times 2})/\sqrt{p_1p_2}}_{w'_{4F}}, \\
& \quad \underbrace{(0, F_{01}c_{01,1})/\sqrt{Tp_2}, \dots, (0, F_{0T}c_{0p_2,1})/\sqrt{Tp_2}}_{w'_{4C}}],
\end{aligned}$$

where  $r_{0i}c'_{0j,1}$ ,  $r_{0i}c'_{0j,2}$  means the first and second row of the matrix  $r_{0i}c'_{0j}$ ,  $w = [w_1, w_2, w_3, w_4]$ . It

is easy to check that  $w'_p w_q = 0$  for  $p \neq q$ . Moreover, we have

$$(p_1 p_2 T)^{\frac{1}{2}} w w' = \begin{pmatrix} \sum_{k=1}^4 w_{kR} w'_{kR} & -\{F_{0t} c_{0j} c_{0j} r'_{0i}\}_{i \leq p_1, t \leq T, j \leq p_2} & -\{F_{0t} c_{0j} r'_{0i} F_{0t}\}_{i \leq p_1, t \leq T, j \leq p_2} \\ -(\{r_{0i} c'_{0j} c'_{0j} F'_{0t}\}_{i \leq p_1, t \leq T, j \leq p_2} & \sum_{k=1}^4 w_{kF} w'_{kF} & -\{r_{0i} c'_{0j} r'_{0i} F'_{0t}\}_{i \leq p_1, t \leq T, j \leq p_2} \\ -\{F'_{0t} r_{0i} c'_{0j} F'_{0t}\}_{i \leq p_1, t \leq T, j \leq p_2} & -\{F'_{0t} r_{0i} c_{0j} r'_{0i}\}_{i \leq p_1, t \leq T, j \leq p_2} & \sum_{k=1}^4 w_{kC} w'_{kC} \end{pmatrix}. \quad (51)$$

Further, it is easy to see that under our normalizations,

$$w w' = \begin{pmatrix} \sigma_{T_1} + \tilde{\sigma}_{T_1} + 1 & 0 & 0 & 0 \\ 0 & \sigma_{T_2} + \tilde{\sigma}_{T_2} + 1 & 0 & 0 \\ 0 & 0 & \sigma_{T_2} + \tilde{\sigma}_{T_2} + 1 & 0 \\ 0 & 0 & 0 & \sigma_{T_1} + \tilde{\sigma}_{T_1} + 1 \end{pmatrix}.$$

Next, we project  $\gamma_k$  onto  $w$ , and write  $\gamma_k = w \beta_k + \zeta_k$ , where  $\beta_k = (w' w)^{-1} w' \gamma_k$ . In particular,

$$\beta_1 = \begin{pmatrix} -\frac{1}{\sigma_{T_1} + \tilde{\sigma}_{T_1} + 1} \\ 0 \\ 0 \\ 0 \end{pmatrix}, \quad \beta_2 = \begin{pmatrix} 0 \\ -\frac{1}{\sigma_{T_2} + \tilde{\sigma}_{T_2} + 1} \\ 0 \\ 0 \end{pmatrix},$$

$$\beta_3 = \begin{pmatrix} 0 \\ 0 \\ -\frac{1}{\sigma_{T_2} + \tilde{\sigma}_{T_2} + 1} \\ -\frac{1}{\sigma_{T_1} + \tilde{\sigma}_{T_1} + 1} \end{pmatrix}, \quad \beta_4 = \begin{pmatrix} 0 \\ 0 \\ -\frac{\sigma_{T_2} + \tilde{\sigma}_{T_2}}{\sigma_{T_2} + \tilde{\sigma}_{T_2} + 1} \\ -\frac{\sigma_{T_1} + \tilde{\sigma}_{T_1}}{\sigma_{T_1} + \tilde{\sigma}_{T_1} + 1} \end{pmatrix}.$$

Define  $B_N = \sum_{k=1}^4 \beta_k \beta'_k$ . It is easy to show that there exists  $\underline{\rho} > 0$  such that  $\rho_{\min}(B_N) > \underline{\rho}$  for all large  $T$  as long as  $\sigma_{T_1} - \sigma_{T_2}$  and  $\tilde{\sigma}_{T_1} - \tilde{\sigma}_{T_2}$  are bounded below by a positive constant for all large  $T$ , which is true under our assumption that  $\sigma_{T_1} \rightarrow \sigma_1$ ,  $\sigma_{T_2} \rightarrow \sigma_2$ ,  $\tilde{\sigma}_{T_1} \rightarrow \tilde{\sigma}_1$ ,  $\tilde{\sigma}_{T_2} \rightarrow \tilde{\sigma}_2$ . It then follows

that

$$\begin{aligned}
\partial^2 \mathbb{P}_{p_1 p_2 T}(\theta_0) / \partial \theta \partial \theta' &= b \left( \sum_{k=1}^4 \gamma_k \gamma'_k \right) = b \cdot w \left( \sum_{k=1}^4 \beta_k \beta'_k \right) w' + b \left( \sum_{k=1}^4 \zeta_k \zeta'_k \right) \\
&= b \underline{\rho} \cdot w w' + b \cdot w (B_N - \underline{\rho} \cdot \mathbb{I}_4) w' + b \left( \sum_{k=1}^4 \zeta_k \zeta'_k \right). \tag{52}
\end{aligned}$$

Now let  $\underline{b} = \min\{\underline{f}, b \underline{\rho}\}$ . Then it follows from (52) that

$$\begin{aligned}
\mathcal{H} &= \partial S^*(\theta_0) / \partial \theta' + \partial^2 \mathbb{P}_{p_1 p_2 T}(\theta_0) / \partial \theta \partial \theta' \\
&= \partial S^*(\theta_0) / \partial \theta' + \underline{b} \cdot w w' + \underbrace{(b \underline{\rho} - \underline{b}) \cdot w w'}_{\geq 0} + \underbrace{b \cdot w (B_N - \underline{\rho} \cdot \mathbb{I}_4) w'}_{\geq 0} + \underbrace{b \left( \sum_{k=1}^4 \zeta_k \zeta'_k \right)}_{\geq 0} \\
&\geq \partial S^*(\theta_0) / \partial \theta' + \underline{b} \cdot w w'.
\end{aligned}$$

Moreover, let

$$\begin{aligned}
S_{d1}^* &= \text{diag} \left[ \left\{ \sum_{t=1}^T \sum_{j=1}^{p_2} \bar{\rho}_{ijt}^{(2)} F_{0t} c_{0j} c'_{0j} F'_{0t} \right\}_{i \leq p_1} \right], S_{d2}^* = \text{diag} \left[ \left\{ \sum_{i=1}^{p_1} \sum_{j=1}^{p_2} \bar{\rho}_{ijt}^{(2)} (r_{0i} c_{0j})^2 \right\}_{t \leq T} \right], \\
S_{d3}^* &= \text{diag} \left[ \left\{ \sum_{i=1}^{p_1} \sum_{t=1}^T \bar{\rho}_{ijt}^{(2)} F'_{0t} r_{0i} r'_{0i} F_{0t} \right\}_{i \leq p_1} \right], S_{d4}^* = \text{diag} \left[ \left\{ \sum_{t=1}^T \sum_{j=1}^{p_2} \bar{\rho}_{ijt}^{(2)} F_{0t} c_{0j} c'_{0j} F'_{0t} \right\}_{i \leq p_1} \right], \\
S_{d5}^* &= \text{diag} \left[ \left\{ \sum_{i=1}^{p_1} \sum_{j=1}^{p_2} \bar{\rho}_{ijt}^{(2)} (r_{0i} c_{0j})^2 \right\}_{t \leq T} \right], S_{d6}^* = \text{diag} \left[ \left\{ \sum_{i=1}^{p_1} \sum_{t=1}^T \bar{\rho}_{ijt}^{(2)} F'_{0t} r_{0i} r'_{0i} F_{0t} \right\}_{i \leq p_1} \right], \\
S_{d7}^* &= \text{diag} \left[ \left\{ \sum_{t=1}^T \sum_{j=1}^{p_2} (\bar{\rho}_{ijt}^{(2)} - \underline{b}) F_{0t} c_{0j} c'_{0j} F'_{0t} \right\}_{i \leq p_1} \right], S_{d8}^* = \text{diag} \left[ \left\{ \sum_{i=1}^{p_1} \sum_{j=1}^{p_2} (\bar{\rho}_{ijt}^{(2)} - \underline{b}) (r_{0i} c_{0j})^2 \right\}_{t \leq T} \right], \\
S_{d9}^* &= \text{diag} \left[ \left\{ \sum_{i=1}^{p_1} \sum_{t=1}^T (\bar{\rho}_{ijt}^{(2)} - \underline{b}) F'_{0t} r_{0i} r'_{0i} F_{0t} \right\}_{i \leq p_1} \right],
\end{aligned}$$

we can write

$$\begin{aligned}
& \partial S^*(\theta_0)/\theta' = (p_1 p_2 T)^{-\frac{1}{2}} \\
& \left( \begin{array}{ccc} S_{d1}^* & \{\bar{\rho}_{ijt}^{(2)} F_{0t} c_{0j} c_{0j} r'_{0i}\} & \{\bar{\rho}_{ijt}^{(2)} F_{0t} c_{0j} r'_{0i} F_{0t}\} \\ \{\bar{\rho}_{ijt}^{(2)} r_{0i} c'_{0j} c'_{0j} F'_{0t}\} & S_{d2}^* & \{\bar{\rho}_{ijt}^{(2)} r_{0i} c'_{0j} r'_{0i} F_{0t}\} \\ \{\bar{\rho}_{ijt}^{(2)} F'_{0t} r_{0i} c'_{0j} F'_{0t}\} & \{\bar{\rho}_{ijt}^{(2)} F'_{0t} r_{0i} c_{0j} r'_{0i}\} & S_{d3}^* \end{array} \right) \\
& = (p_1 p_2 T)^{-\frac{1}{2}} \underline{b} \underbrace{\left( \begin{array}{ccc} S^* d 4 \mathbf{0}_{(2p_2 \times T) \cdot (2p_1 \times 2p_2)} & \mathbf{0}_{2Tp_1 \times 2Tp_2} & \\ \mathbf{0}_{(2p_2 \times 2p_1) \cdot (T \times 2p_2)} & S_{d5}^* & \mathbf{0}_{(2p_2 \times 2p_1) \cdot (T \times 2p_1)} \\ \mathbf{0}_{2Tp_2 \times 2Tp_1} & \mathbf{0}_{(2p_1 \times T) \cdot (2p_1 \times 2p_2)} & S_{d6}^* \end{array} \right)}_I \\
& + (p_1 p_2 T)^{-\frac{1}{2}} \underline{b} \underbrace{\left( \begin{array}{ccc} \mathbf{0}_{2p_1 \times 2p_1} & \{\bar{\rho}_{ijt}^{(2)} F_{0t} c_{0j} c_{0j} r'_{0i}\} & \{\bar{\rho}_{ijt}^{(2)} F_{0t} c_{0j} r'_{0i} F_{0t}\} \\ \{\bar{\rho}_{ijt}^{(2)} r_{0i} c'_{0j} c'_{0j} F'_{0t}\} & \mathbf{0}_{(2 \times 2)^2 \cdot T} & \{\bar{\rho}_{ijt}^{(2)} r_{0i} c'_{0j} r'_{0i} F_{0t}\} \\ \{\bar{\rho}_{ijt}^{(2)} F'_{0t} r_{0i} c'_{0j} F'_{0t}\} & \{\bar{\rho}_{ijt}^{(2)} F'_{0t} r_{0i} c_{0j} r'_{0i}\} & \mathbf{0}_{2p_2 \times 2p_2} \end{array} \right)}_{II} \\
& + (p_1 p_2 T)^{-\frac{1}{2}} \underbrace{\left( \begin{array}{ccc} S_{d7}^* & \{(\bar{\rho}_{ijt}^{(2)} - \underline{b}) F_{0t} c_{0j} c_{0j} r'_{0i}\} & \{(\bar{\rho}_{ijt}^{(2)} - \underline{b}) F_{0t} c_{0j} r'_{0i} F_{0t}\} \\ \{(\bar{\rho}_{ijt}^{(2)} - \underline{b}) r_{0i} c'_{0j} c'_{0j} F'_{0t}\} & S_{d8}^* & \{(\bar{\rho}_{ijt}^{(2)} - \underline{b}) r_{0i} c'_{0j} r'_{0i} F_{0t}\} \\ \{(\bar{\rho}_{ijt}^{(2)} - \underline{b}) F'_{0t} r_{0i} c'_{0j} F'_{0t}\} & \{(\bar{\rho}_{ijt}^{(2)} - \underline{b}) F'_{0t} r_{0i} c_{0j} r'_{0i}\} & S_{d9}^* \end{array} \right)}_{III}.
\end{aligned}$$

Note that by our Assumptions 1 and 2, there exists a constant  $c > 0$  such that

$$\begin{aligned}
& I \\
& = \underline{b} \left( \begin{array}{ccc} \sqrt{Tp_2/p_1} \mathbb{I}_{p_1} \otimes \text{diag}(\sigma_{T_1}, \sigma_{T_2}) & \mathbf{0}_{(2p_2 \times T) \cdot (2p_1 \times 2p_2)} & \mathbf{0}_{2Tp_1 \times 2Tp_2} \\ \mathbf{0}_{(2p_2 \times 2p_1) \cdot (T \times 2p_2)} & \sqrt{p_1 p_2 / T} \mathbb{I}_T \otimes (\mathbb{I}_2 * \mathbb{I}_2) & \mathbf{0}_{(2p_2 \times 2p_1) \cdot (T \times 2p_1)} \\ \mathbf{0}_{2Tp_2 \times 2Tp_1} & \mathbf{0}_{(2p_1 \times T) \cdot (2p_1 \times 2p_2)} & \sqrt{Tp_1/p_2} \mathbb{I}_{p_2} \otimes \text{diag}(\tilde{\sigma}_{T_1}, \tilde{\sigma}_{T_2}) \end{array} \right) \\
& \geq \underline{c} \cdot \mathbb{I}.
\end{aligned} \tag{53}$$

From (51), we have

$$II + \underline{b} \cdot ww' = \underline{b} \cdot \begin{pmatrix} \sum_{k=1}^4 w_{kR} w'_{kR} & \mathbf{0}_{(2p_2 \times T) \cdot (2p_1 \times 2p_2)} & \mathbf{0}_{2Tp_1 \times 2Tp_2} \\ \mathbf{0}_{(2p_2 \times 2p_1) \cdot (T \times 2p_2)} & \sum_{k=1}^4 w_{kF} w'_{kF} & \mathbf{0}_{(2p_2 \times 2p_1) \cdot (T \times 2p_1)} \\ \mathbf{0}_{2Tp_2 \times 2Tp_1} & \mathbf{0}_{(2p_1 \times T) \cdot (2p_1 \times 2p_2)} & \sum_{k=1}^4 w_{kC} w'_{kC} \end{pmatrix} \geq 0. \quad (54)$$

For the last term, we have, for  $p_1, p_2, T$  large enough,

$$III = \frac{1}{\sqrt{p_1 p_2 T}} \sum_{i=1}^{p_1} \sum_{t=1}^T \sum_{j=1}^{p_2} (\bar{\rho}_{ijt}^{(2)} - \underline{b}) \mu_{ijt} \mu'_{ijt} \geq 0, \quad (55)$$

where  $\mu_{ijt} = [0_{1 \times 2}, \dots, c'_{0j} F'_{0t}, \dots, 0_{1 \times 2}, 0_{2 \times 2}, \dots, c_{0j} r'_{0i}, \dots, 0_{2 \times 2}, 0_{1 \times 2}, \dots, r'_{0i} F_{0t}, \dots, 0_{1 \times 2}]'$ , because Assumption 1 and Lemma S.1 imply that  $\bar{\rho}_{ijt}^{(2)} \geq \underline{f}$  for all  $i, j, t$ . It then follows from (53), (54), and (55) that

$$\mathcal{H} \geq \partial S^*(\theta_0)/\theta' + \underline{b} \cdot ww' = I + II + III + \underline{b} \cdot ww' \geq \underline{c} \cdot \mathbb{I},$$

and thus

$$\mathcal{H}^{-1} \leq \underline{c}^{-1} \cdot \mathbb{I}. \quad (56)$$

Finally, write  $\mathcal{H} = \mathcal{H}_d + \mathcal{C}$ , where

$$\mathcal{C} = \begin{pmatrix} \mathbf{0}_{2p_1 \times 2p_1} & \{\bar{\rho}_{ijt}^{(2)} F_{0t} c_{0j} c_{0j} r'_{0i}\}_{i \leq p_1, t \leq T, j \leq p_2} & \{\bar{\rho}_{ijt}^{(2)} F_{0t} c_{0j} r'_{0i} F_{0t}\}_{i \leq p_1, t \leq T, j \leq p_2} \\ \{\bar{\rho}_{ijt}^{(2)} r_{0i} c'_{0j} c'_{0j} F'_{0t}\}_{i \leq p_1, t \leq T, j \leq p_2} & \mathbf{0}_{(2 \times 2)^2 T} & \{\bar{\rho}_{ijt}^{(2)} r_{0i} c'_{0j} r'_{0i} F_{0t}\}_{i \leq p_1, t \leq T, j \leq p_2} \\ \{\bar{\rho}_{ijt}^{(2)} F'_{0t} r_{0i} c'_{0j} F'_{0t}\}_{i \leq p_1, t \leq T, j \leq p_2} & \{\bar{\rho}_{ijt}^{(2)} F'_{0t} r_{0i} c_{0j} r'_{0i}\}_{i \leq p_1, t \leq T, j \leq p_2} & \mathbf{0}_{2p_2 \times 2p_2} \end{pmatrix} + b \left( \sum_{k=1}^4 \gamma_k \gamma'_k \right).$$

Note that  $\mathcal{H}^{-1} - \mathcal{H}_d^{-1} = -\mathcal{H}_d^{-1} \mathcal{C} \mathcal{H}_d^{-1} + \mathcal{H}_d^{-1} \mathcal{C} \mathcal{H}^{-1} \mathcal{C} \mathcal{H}_d^{-1}$ , and thus  $\|\mathcal{H}^{-1} - \mathcal{H}_d^{-1}\|_{\max} \leq \|\mathcal{H}_d^{-1} \mathcal{C} \mathcal{H}_d^{-1}\|_{\max} + \|\mathcal{H}_d^{-1} \mathcal{C} \mathcal{H}^{-1} \mathcal{C} \mathcal{H}_d^{-1}\|_{\max}$ . Inequality (56) implies that  $\mathcal{H}_d^{-1} \mathcal{C} \mathcal{H}^{-1} \mathcal{C} \mathcal{H}_d^{-1} \leq \underline{c} \mathcal{H}_d^{-1} \mathcal{C}^2 \mathcal{H}^{-1}$ , and thus the  $j$ th diagonal element of  $\mathcal{H}_d^{-1} \mathcal{C} \mathcal{H}^{-1} \mathcal{C} \mathcal{H}_d^{-1}$  is smaller than the  $j$ th diagonal element of  $\underline{c} \mathcal{H}_d^{-1} \mathcal{C}^2 \mathcal{H}^{-1}$ . It then follows that  $\|\mathcal{H}_d^{-1} \mathcal{C} \mathcal{H}^{-1} \mathcal{C} \mathcal{H}_d^{-1}\|_{\max} \leq \underline{c} \|\mathcal{H}_d^{-1} \mathcal{C}^2 \mathcal{H}^{-1}\|_{\max}$  and therefore

$$\|\mathcal{H}^{-1} - \mathcal{H}_d^{-1}\|_{\max} \leq \|\mathcal{H}_d^{-1} \mathcal{C} \mathcal{H}_d^{-1}\|_{\max} + \underline{c} \|\mathcal{H}_d^{-1} \mathcal{C}^2 \mathcal{H}_d^{-1}\|_{\max}$$

because the entry with the largest absolute value of a positive semidefinite matrix is always on the diagonal. Since  $\mathcal{H}_d^{-1}$  is a block-diagonal matrix whose elements are all  $O(1)$  by Assumption 2, and both  $\mathcal{C}_{\max}$  and  $\mathcal{C}_{\max}^2$  can be shown to be  $O(1/Tp_2)$ , then the desired result follows.  $\square$

Since  $\partial \mathbb{P}_{p_1 p_2 T}(\tilde{\theta})/\partial \theta = \partial \mathbb{P}_{p_1 p_2 T}(\theta_0)/\partial \theta = 0$ , (50) implies that

$$\tilde{\theta} - \theta_0 = \mathcal{H}^{-1} S^*(\tilde{\theta}) - \mathcal{H}^{-1} S^*(\theta_0) - 0.5 \mathcal{H}^{-1} \mathcal{R}(\tilde{\theta}). \quad (57)$$

Define

$$S_{p_1 p_2 T}^*(\theta) = \left[ \dots, -\frac{1}{\sqrt{p_1 p_2 T}} \sum_{t=1}^T \sum_{j=1}^{p_2} \rho^{(1)}(X_{ijt} - r'_i F_t c_j) F_t c_j, \dots, \dots, \right. \\ \left. -\frac{1}{\sqrt{p_1 p_2 T}} \sum_{t=1}^T \sum_{j=1}^{p_2} \rho^{(1)}(X_{ijt} - r'_i F_t c_j) r_i c'_j, \dots, \dots, -\frac{1}{\sqrt{p_1 p_2 T}} \sum_{t=1}^T \sum_{j=1}^{p_2} \rho^{(1)}(X_{ijt} - r'_i F_t c_j) F'_t r_i, \dots \right],$$

$\tilde{S}^*(\theta) = S_{p_1 p_2 T}^*(\theta) - S^*(\theta)$ , and  $\mathcal{D} = \mathcal{H}^{-1} - \mathcal{H}_d^{-1}$ .  $\mathcal{D}$  can be written as a block matrix as

$$\mathcal{D} = \begin{pmatrix} \mathcal{D}^{RR} & \mathcal{D}^{RF} & \mathcal{D}^{RC} \\ \mathcal{D}^{FR} & \mathcal{D}^{FF} & \mathcal{D}^{FC} \\ \mathcal{D}^{CR} & \mathcal{D}^{CF} & \mathcal{D}^{CC} \end{pmatrix},$$

where the components of  $\mathcal{D}^{RR}$  is  $k_1 \times k_1$  matrix with  $p_1$  ‘block rows’ and  $p_1$  ‘block columns’, the components of  $\mathcal{D}^{RF}$  is  $\frac{\partial k_1}{\partial(k_1 \times k_2)}$  three dimensional matrix with  $p_1$  ‘block rows’ and  $T$  ‘block columns’, the components of  $\mathcal{D}^{RC}$  is  $k_1 \times k_2$  matrix with  $p_1$  ‘block rows’ and  $p_2$  ‘block columns’, the components of  $\mathcal{D}^{FR}$  is  $\frac{\partial(k_1 \times k_2)}{\partial k_1}$  three dimensional matrix with  $T$  ‘block rows’ and  $p_1$  ‘block columns’, the components of  $\mathcal{D}^{FF}$  is  $\frac{\partial(k_1 \times k_2)}{\partial(k_1 \times k_2)}$  three dimensional matrix with  $T$  ‘block rows’ and  $T$  ‘block columns’, the components of  $\mathcal{D}^{FC}$  is  $\frac{\partial(k_1 \times k_2)}{\partial k_2}$  three dimensional matrix with  $T$  ‘block rows’ and  $p_2$  ‘block columns’, the components of  $\mathcal{D}^{CR}$  is  $k_2 \times k_1$  matrix with  $p_2$  ‘block rows’ and  $p_1$  ‘block columns’, the components of  $\mathcal{D}^{CF}$  is  $\frac{\partial k_2}{\partial(k_1 \times k_2)}$  three dimensional matrix with  $p_2$  ‘block rows’ and  $T$  ‘block columns’, the components of  $\mathcal{D}^{CC}$  is  $k_2 \times k_2$  matrix with  $p_2$  ‘block rows’ and  $p_2$  ‘block columns’. Write  $\mathcal{D}_{t,l}^{FR}$  as the  $t$ th ‘block row’ and  $l$ th ‘block column’ of  $\mathcal{D}^{FR}$ ,  $\mathcal{D}_{t,s}^{FF}$  as the  $t$ th ‘block row’ and  $s$ th ‘block column’ of  $\mathcal{D}^{FF}$ ,  $\mathcal{D}_{t,k}^{FC}$  as the  $t$ th ‘block row’ and  $k$ th ‘block column’ of  $\mathcal{D}^{FC}$ .

$$\mathcal{D}^{RR} = \begin{pmatrix} \overbrace{k_1 \times k_1 \ \dots \ k_1 \times k_1}^{p_1} \\ \vdots \\ k_1 \times k_1 \ \dots \ k_1 \times k_1 \end{pmatrix} p_1, \quad \mathcal{D}^{RF} = \begin{pmatrix} \overbrace{\frac{\partial k_1}{\partial(k_1 \times k_2)} \ \dots \ \frac{\partial k_1}{\partial(k_1 \times k_2)}}^T \\ \vdots \\ \frac{\partial k_1}{\partial(k_1 \times k_2)} \ \dots \ \frac{\partial k_1}{\partial(k_1 \times k_2)} \end{pmatrix} p_1,$$

$$\mathcal{D}^{RC} = \begin{pmatrix} \overbrace{k_1 \times k_2 \ \dots \ k_1 \times k_2}^{p_2} \\ \vdots \\ k_1 \times k_2 \ \dots \ k_1 \times k_2 \end{pmatrix} p_1, \quad \mathcal{D}^{FR} = \begin{pmatrix} \overbrace{\frac{\partial(k_1 \times k_2)}{\partial k_1} \ \dots \ \frac{\partial(k_1 \times k_2)}{\partial k_1}}^{p_1} \\ \vdots \quad \frac{\partial(k_1 \times k_2)}{\partial k_1} \quad \vdots \\ \frac{\partial(k_1 \times k_2)}{\partial k_1} \ \dots \ \frac{\partial(k_1 \times k_2)}{\partial k_1} \end{pmatrix} T, \quad \text{with } t, l$$

$$\mathcal{D}^{FF} = \begin{pmatrix} \overbrace{\frac{\partial(k_1 \times k_2)}{\partial(k_1 \times k_2)} \ \dots \ \frac{\partial(k_1 \times k_2)}{\partial(k_1 \times k_2)}}^T \\ \vdots \quad \frac{\partial(k_1 \times k_2)}{\partial(k_1 \times k_2)} \quad \vdots \\ \frac{\partial(k_1 \times k_2)}{\partial(k_1 \times k_2)} \ \dots \ \frac{\partial(k_1 \times k_2)}{\partial(k_1 \times k_2)} \end{pmatrix} T, \quad \mathcal{D}^{FC} = \begin{pmatrix} \overbrace{\frac{\partial(k_1 \times k_2)}{\partial k_2} \ \dots \ \frac{\partial(k_1 \times k_2)}{\partial k_2}}^{p_2} \\ \vdots \quad \frac{\partial(k_1 \times k_2)}{\partial k_2} \quad \vdots \\ \frac{\partial(k_1 \times k_2)}{\partial k_2} \ \dots \ \frac{\partial(k_1 \times k_2)}{\partial k_2} \end{pmatrix} T, \quad \text{with } t, k$$

$$\mathcal{D}^{CR} = \begin{pmatrix} \overbrace{k_2 \times k_1 \ \dots \ k_2 \times k_1}^{p_1} \\ \vdots \\ k_2 \times k_1 \ \dots \ k_2 \times k_1 \end{pmatrix} p_2, \quad \mathcal{D}^{CF} = \begin{pmatrix} \overbrace{\frac{\partial k_2}{\partial(k_1 \times k_2)} \ \dots \ \frac{\partial k_2}{\partial(k_1 \times k_2)}}^T \\ \vdots \\ \frac{\partial k_2}{\partial(k_1 \times k_2)} \ \dots \ \frac{\partial k_2}{\partial(k_1 \times k_2)} \end{pmatrix} p_2,$$

$$\mathcal{D}^{CC} = \begin{pmatrix} \overbrace{k_2 \times k_2 \ \dots \ k_2 \times k_2}^{p_2} \\ \vdots \\ k_2 \times k_2 \ \dots \ k_2 \times k_2 \end{pmatrix} p_2.$$

Note that by the first-order conditions,  $S_{p_1 p_2 T}^*(\tilde{\theta}) = 0$ . As a result, we can write

$$\begin{aligned}
\mathcal{H}^{-1}S^*(\tilde{\theta}) &= \mathcal{H}_d^{-1}S^*(\tilde{\theta}) + \mathcal{D}S^*(\tilde{\theta}) = -\mathcal{H}_d^{-1}\tilde{S}^*(\tilde{\theta}) + \mathcal{D}S^*(\tilde{\theta}) \\
&= -\mathcal{H}_d^{-1}\tilde{S}^*(\theta_0) - \mathcal{H}_d^{-1}(\tilde{S}^*(\tilde{\theta}) - \tilde{S}^*(\theta_0)) + \mathcal{D}S^*(\tilde{\theta}) \\
&= -\mathcal{H}_d^{-1}\tilde{S}^*(\theta_0) - \mathcal{H}_d^{-1}(\tilde{S}^*(\tilde{\theta}) - \tilde{S}^*(\theta_0)) \\
&\quad -\mathcal{D}\tilde{S}^*(\theta_0) - \mathcal{D}(\tilde{S}^*(\tilde{\theta}) - \tilde{S}^*(\theta_0)).
\end{aligned} \tag{58}$$

Next, let  $\mathcal{R}(\tilde{\theta})_i$  denote the vector containing the  $(i-1)k_1 + 1$ th to the  $ik_1$ th elements of  $\mathcal{R}(\tilde{\theta})$  for  $i = 1, \dots, p_1$ ,  $\mathcal{R}(\tilde{\theta})_{p_1+t}$  denote the  $(p_1+t-1)k_1 + 1$ th rows to the  $(p_1+t)k_1$ th rows and  $(p_1+t-1)k_2 + 1$ th columns to the  $(p_1+t)k_2$ th columns of  $\mathcal{R}(\tilde{\theta})$  for  $t = 1, \dots, T$ ,  $\mathcal{R}(\tilde{\theta})_{p_1+T+j}$  denote the vector containing the  $(p_1+T+j-1)k_2 + 1$ th to the  $(p_1+T+j)k_2$ th elements of  $\mathcal{R}(\tilde{\theta})$  for  $j = 1, \dots, p_2$ . Let  $\bar{O}_p(\cdot)$  denote a stochastic order that is uniformly in  $i, j$  and  $t$ . Then, by the result of Lemma F.3, it can be shown that

$$\mathcal{R}(\tilde{\theta})_i = \bar{O}_p(1)\|\tilde{r}_i - r_{0i}\|^2 + \bar{O}_p(1/\sqrt{Tp_2})\|\tilde{r}_i - r_{0i}\| + \bar{O}_p(1/Tp_2) \tag{59}$$

for  $i = 1, \dots, p_1$ , and

$$\mathcal{R}(\tilde{\theta})_{p_1+t} = \bar{O}_p(1)\|\tilde{F}_t - F_{0t}\|^2 + \bar{O}_p(1/\sqrt{Tp_2})\|\tilde{F}_t - F_{0t}\| + \bar{O}_p(1/Tp_2) \tag{60}$$

for  $t = 1, \dots, T$ , and

$$\mathcal{R}(\tilde{\theta})_{p_1+T+j} = \bar{O}_p(1)\|\tilde{c}_j - c_{0j}\|^2 + \bar{O}_p(1/\sqrt{Tp_2})\|\tilde{c}_j - c_{0j}\| + \bar{O}_p(1/Tp_2) \tag{61}$$

for  $j = 1, \dots, p_2$ .

Note that Lemma F.1 and Lemma F.6 imply that  $\|\mathcal{H}^{-1}S^*(\theta_0)\|_{max} = \bar{O}(h^m)$ . Then, from (57)

to (61), we can write

$$\begin{aligned}
\tilde{F}_t - F_{0t} &= (\Psi_{p_1 p_2, t})^{-1} \frac{1}{p_1 p_2} \sum_{l=1}^{p_1} \sum_{k=1}^{p_2} \tilde{\rho}_{l t k}^{(1)} r_{0l} c'_{0k} + \frac{1}{\sqrt{p_1 p_2 T}} \sum_{l=1}^{p_1} \sum_{s=1}^T \sum_{k=1}^{p_2} \mathcal{D}_{t,l}^{FR} \cdot \tilde{\rho}_{l s k}^{(1)} \cdot F_{0s} c_{0k} \\
&+ \frac{1}{\sqrt{p_1 p_2 T}} \sum_{l=1}^{p_1} \sum_{s=1}^T \sum_{k=1}^{p_2} \mathcal{D}_{t,s}^{FF} \cdot \tilde{\rho}_{l s k}^{(1)} \cdot r_{0l} c'_{0k} + \frac{1}{\sqrt{p_1 p_2 T}} \sum_{l=1}^{p_1} \sum_{s=1}^T \sum_{k=1}^{p_2} \mathcal{D}_{t,k}^{FC} \cdot \tilde{\rho}_{l s k}^{(1)} \cdot F'_{0s} r_{0l} \\
&+ (\Psi_{p_1 p_2, t})^{-1} \frac{1}{p_1 p_2} \sum_{l=1}^{p_1} \sum_{k=1}^{p_2} \{ \tilde{\rho}^{(1)}(X_{l t k} - \tilde{r}'_l \tilde{F}_t \tilde{c}_k) \tilde{r}_l \tilde{c}'_k - \tilde{\rho}_{l t k}^{(1)} r_{0l} c'_{0k} \} \\
&+ \frac{1}{\sqrt{p_1 p_2 T}} \sum_{l=1}^{p_1} \sum_{s=1}^T \sum_{k=1}^{p_2} \mathcal{D}_{t,l}^{FR} \{ \tilde{\rho}^{(1)}(X_{l s k} - \tilde{r}'_l \tilde{F}_s \tilde{c}_k) \tilde{F}_s \tilde{c}_k - \tilde{\rho}_{l s k}^{(1)} F_{0s} c_{0k} \} \\
&+ \frac{1}{\sqrt{p_1 p_2 T}} \sum_{l=1}^{p_1} \sum_{s=1}^T \sum_{k=1}^{p_2} \mathcal{D}_{t,s}^{FF} \{ \tilde{\rho}^{(1)}(X_{l s k} - \tilde{r}'_l \tilde{F}_s \tilde{c}_k) \tilde{r}_l \tilde{c}'_k - \tilde{\rho}_{l s k}^{(1)} r_{0l} c'_{0k} \} \\
&+ \frac{1}{\sqrt{p_1 p_2 T}} \sum_{l=1}^{p_1} \sum_{s=1}^T \sum_{k=1}^{p_2} \mathcal{D}_{t,k}^{FC} \{ \tilde{\rho}^{(1)}(X_{l s k} - \tilde{r}'_l \tilde{F}_s \tilde{c}_k) \tilde{F}'_s \tilde{r}_l - \tilde{\rho}_{l s k}^{(1)} F'_{0s} r_{0l} \} \\
&- 0.5 (\Psi_{p_1 p_2, t})^{-1} \mathcal{R}(\tilde{\theta})_{p_1+t} - 0.5 \sum_{l=1}^{p_1} \mathcal{D}_{t,l}^{FR} \mathcal{R}(\tilde{\theta})_l - 0.5 \sum_{s=1}^T \mathcal{D}_{t,s}^{FF} \mathcal{R}(\tilde{\theta})_{p_1+s} \\
&- 0.5 \sum_{k=1}^{p_2} \mathcal{D}_{t,k}^{FC} \mathcal{R}(\tilde{\theta})_{p_1+T+k} + \bar{O}(h^m). \tag{62}
\end{aligned}$$

$$\begin{aligned}
\tilde{c}_j - c_{0j} &= (\varphi_{T p_1, j})^{-1} \frac{1}{T p_1} \sum_{l=1}^{p_1} \sum_{s=1}^T \tilde{\rho}_{l s j}^{(1)} F'_{0s} r_{0l} + \frac{1}{\sqrt{p_1 p_2 T}} \sum_{l=1}^{p_1} \sum_{s=1}^T \sum_{k=1}^{p_2} \mathcal{D}_{j,l}^{CR} \tilde{\rho}_{l s k}^{(1)} F_{0s} c_{0k} \\
&+ \frac{1}{\sqrt{p_1 p_2 T}} \sum_{l=1}^{p_1} \sum_{s=1}^T \sum_{k=1}^{p_2} \mathcal{D}_{j,s}^{CF} \tilde{\rho}_{l s k}^{(1)} \cdot r_{0l} c'_{0k} + \frac{1}{\sqrt{p_1 p_2 T}} \sum_{l=1}^{p_1} \sum_{s=1}^T \sum_{k=1}^{p_2} \mathcal{D}_{j,k}^{CC} \tilde{\rho}_{l s k}^{(1)} F'_{0s} r_{0l} \\
&+ (\varphi_{T p_1, j})^{-1} \frac{1}{T p_1} \sum_{l=1}^{p_1} \sum_{s=1}^T \{ \tilde{\rho}^{(1)}(X_{l s j} - \tilde{r}'_l \tilde{F}_s \tilde{c}_j) \tilde{F}_s \tilde{r}_l - \tilde{\rho}_{l s j}^{(1)} F'_{0s} r_{0l} \} \\
&+ \frac{1}{\sqrt{p_1 p_2 T}} \sum_{l=1}^{p_1} \sum_{s=1}^T \sum_{k=1}^{p_2} \mathcal{D}_{j,l}^{CR} \{ \tilde{\rho}^{(1)}(X_{l s k} - \tilde{r}'_l \tilde{F}_s \tilde{c}_k) \tilde{F}_s \tilde{c}_k - \tilde{\rho}_{l s k}^{(1)} F_{0s} c_{0k} \} \\
&+ \frac{1}{\sqrt{p_1 p_2 T}} \sum_{l=1}^{p_1} \sum_{s=1}^T \sum_{k=1}^{p_2} \mathcal{D}_{j,s}^{CF} \{ \tilde{\rho}^{(1)}(X_{l s k} - \tilde{r}'_l \tilde{F}_s \tilde{c}_k) \tilde{r}_l \tilde{c}'_k - \tilde{\rho}_{l s k}^{(1)} r_{0l} c'_{0k} \} \\
&+ \frac{1}{\sqrt{p_1 p_2 T}} \sum_{l=1}^{p_1} \sum_{s=1}^T \sum_{k=1}^{p_2} \mathcal{D}_{j,k}^{CC} \{ \tilde{\rho}^{(1)}(X_{l s k} - \tilde{r}'_l \tilde{F}_s \tilde{c}_k) \tilde{F}'_s \tilde{r}_l - \tilde{\rho}_{l s k}^{(1)} F'_{0s} r_{0l} \} \\
&- 0.5 (\varphi_{T p_1, j})^{-1} \mathcal{R}(\tilde{\theta})_{p_1+T+j} - 0.5 \sum_{l=1}^{p_1} \mathcal{D}_{j,l}^{CR} \mathcal{R}(\tilde{\theta})_l - 0.5 \sum_{s=1}^T \mathcal{D}_{j,s}^{CF} \mathcal{R}(\tilde{\theta})_{p_1+s} \\
&- 0.5 \sum_{k=1}^{p_2} \mathcal{D}_{j,k}^{CC} \mathcal{R}(\tilde{\theta})_{p_1+T+k} + \bar{O}(h^m).
\end{aligned}$$

**Lemma F.7.** Let  $c_1, \dots, c_T$  and  $d_1, \dots, d_{p_2}$  be sequence of uniformly bounded constants. Then, under Assumptions 1 and 2, we have

$$\frac{1}{T} \sum_{t=1}^T c_t (\tilde{F}_t - F_{0t}) = O_p\left(\frac{1}{Tp_2h}\right), \quad \frac{1}{p_2} \sum_{j=1}^{p_2} d_j (\tilde{c}_j - c_{0j}) = O_p\left(\frac{1}{Tp_2h}\right).$$

*Proof.* Define  $a_l = \frac{\sqrt{p_1 p_2 T}}{T} \sum_{t=1}^T c_t \mathcal{D}_{t,l}^{FR}$ , for  $l = 1, \dots, p_1$ ,  $a_s = \frac{\sqrt{p_1 p_2 T}}{T} \sum_{t=1}^T c_t \mathcal{D}_{t,s}^{FF}$ , for  $s = 1, \dots, T$ ,  $a_k = \frac{\sqrt{p_1 p_2 T}}{T} \sum_{t=1}^T c_t \mathcal{D}_{t,k}^{FC}$ , for  $k = 1, \dots, p_2$ . Lemma F.6 implies that  $\max_{1 \leq l \leq p_1} \|a_l\|$ ,  $\max_{1 \leq s \leq T} \|a_s\|$  and  $\max_{1 \leq k \leq p_2} \|a_k\|$  are bounded. From (62), we have

$$\begin{aligned} & \frac{1}{T} \sum_{t=1}^T c_t (\tilde{F}_t - F_{0t}) \\ &= \frac{1}{Tp_1 p_2} \sum_{t=1}^T \sum_{l=1}^{p_1} \sum_{k=1}^{p_2} c_t (\Psi_{p_1 p_2, t})^{-1} \tilde{\rho}_{ltk}^{(1)} r_{0l} c'_{0k} + \frac{1}{p_1 p_2 T} \sum_{l=1}^{p_1} \sum_{s=1}^T \sum_{k=1}^{p_2} a_l \tilde{\rho}_{lsk}^{(1)} F_{0s} c_{0k} \\ &+ \frac{1}{p_1 p_2 T} \sum_{l=1}^{p_1} \sum_{s=1}^T \sum_{k=1}^{p_2} a_s \tilde{\rho}_{lsk}^{(1)} r_{0l} c'_{0k} + \frac{1}{p_1 p_2 T} \sum_{l=1}^{p_1} \sum_{s=1}^T \sum_{k=1}^{p_2} a_k \tilde{\rho}_{lsk}^{(1)} F'_{0s} r_{0l} \\ &+ \frac{1}{Tp_1 p_2} \sum_{l=1}^{p_1} \sum_{t=1}^T \sum_{k=1}^{p_2} c_t (\psi_{p_1 p_2, t})^{-1} \{ \tilde{\rho}^{(1)}(X_{ltk} - \tilde{r}_l \tilde{F}_t \tilde{c}_k) \tilde{r}_l \tilde{c}'_k - \tilde{\rho}_{ltk}^{(1)} r_{0l} c_{0k} \} \\ &+ \frac{1}{p_1 p_2 T} \sum_{l=1}^{p_1} \sum_{s=1}^T \sum_{k=1}^{p_2} a_l \{ \tilde{\rho}^{(1)}(X_{lsk} - \tilde{r}_l \tilde{F}_s \tilde{c}_k) \tilde{F}_s \tilde{c}_k - \tilde{\rho}_{lsk}^{(1)} F_{0s} c_{0k} \} \\ &+ \frac{1}{p_1 p_2 T} \sum_{l=1}^{p_1} \sum_{s=1}^T \sum_{k=1}^{p_2} a_s \{ \tilde{\rho}^{(1)}(X_{lsk} - \tilde{r}_l \tilde{F}_s \tilde{c}_k) \tilde{r}_l \tilde{c}'_k - \tilde{\rho}_{lsk}^{(1)} r_{0l} c'_{0k} \} \\ &+ \frac{1}{p_1 p_2 T} \sum_{l=1}^{p_1} \sum_{s=1}^T \sum_{k=1}^{p_2} a_k \{ \tilde{\rho}^{(1)}(X_{lsk} - \tilde{r}_l \tilde{F}_s \tilde{c}_k) \tilde{F}'_s \tilde{r}_l - \tilde{\rho}_{lsk}^{(1)} F'_{0s} r_{0l} \} \\ &- 0.5 \frac{1}{T} \sum_{t=1}^T c_t (\Psi_{p_1 p_2, t})^{-1} \mathcal{R}(\tilde{\theta})_{p_1+t} - 0.5 \frac{1}{\sqrt{p_1 p_2 T}} \sum_{l=1}^{p_1} a_l \mathcal{R}(\tilde{\theta})_l \\ &- 0.5 \frac{1}{\sqrt{p_1 p_2 T}} \sum_{s=1}^T a_s \mathcal{R}(\tilde{\theta})_{p_1+s} - 0.5 \frac{1}{\sqrt{p_1 p_2 T}} \sum_{k=1}^{p_2} a_k \mathcal{R}(\tilde{\theta})_{p_1+T+k} + \bar{O}(h^m). \end{aligned} \quad (63)$$

First, by Lyapunov's CLT, it is easy to see that the first three terms on the RHS of (63) are all  $O_p(1/\sqrt{p_1 p_2 T})$ .

Next, it follows from Lemma F.3, (59), (60), (61) and Assumption 2(v) that the last four terms on the RHS of (63) are all  $O_p(1/L_{p_1 p_2 T}^2)$ . Finally, we will show that the remaining three terms on the RHS of (63) are all  $O_p(1/(Tp_2h))$ , from which the desired result follows.

Define

$$\mathbb{V}_{p_1 p_2 T}(\theta) = \frac{1}{p_1 p_2 T} \sum_{l=1}^{p_1} \sum_{s=1}^T \sum_{k=1}^{p_2} a_l \{ \tilde{\rho}^{(1)}(X_{lsk} - \tilde{r}'_l \tilde{F}_s \tilde{c}_k) \tilde{F}_s \tilde{c}_k - \tilde{\rho}_{lsk}^{(1)} F_{0s} c_{0k} \},$$

and  $\Delta_{p_1 p_2 T}(\theta_a, \theta_b) = \sqrt{p_1 p_2 T} h [\mathbb{V}_{p_1 p_2 T}(\theta_a) - \mathbb{V}_{p_1 p_2 T}(\theta_b)]$ . Note that

$$\begin{aligned} \Delta_{p_1 p_2 T}(\theta_a, \theta_b) &= \underbrace{\frac{h}{\sqrt{p_1 p_2 T}} \sum_{l=1}^{p_1} \sum_{s=1}^T \sum_{k=1}^{p_2} a_l \cdot \tilde{\rho}^{(1)}(X_{lsk} - r'_{al} F_{as} c_{ak}) \cdot (F_{as} c_{ak} - F_{bs} c_{bk})}_{\Delta_{1, p_1 p_2 T}(\theta_a, \theta_b)} \\ &\quad + \underbrace{\frac{h}{\sqrt{p_1 p_2 T}} \sum_{l=1}^{p_1} \sum_{s=1}^T \sum_{k=1}^{p_2} a_l \cdot [\tilde{\rho}^{(1)}(X_{lsk} - r'_{al} F_{as} c_{ak}) - \tilde{\rho}^{(1)}(X_{lsk} - r'_{bl} F_{bs} c_{bk})] \cdot F_{bs} c_{bk}}_{\Delta_{2, p_1 p_2 T}(\theta_a, \theta_b)}. \end{aligned}$$

Lemma F.1 implies that

$$\begin{aligned} h |a_l \cdot \tilde{\rho}^{(1)}(X_{lsk} - r'_{al} F_{as} c_{ak}) \cdot (F_{as} c_{ak} - F_{bs} c_{bk})| &\lesssim |r'_{al} F_{as} c_{ak} - r'_{bl} F_{bs} c_{bk}|, \\ h |\rho^{(1)}(X_{lsk} - r'_{al} F_{as} c_{ak}) - \rho^{(1)}(X_{lsk} - r'_{bl} F_{bs} c_{bk})| &\lesssim |r'_{al} F_{as} c_{ak} - r'_{bl} F_{bs} c_{bk}|. \end{aligned}$$

By Hoeffding's inequality and Lemma 2.2.1 of [4], we can show that for  $d(\theta_a, \theta_b)$  sufficiently small,

$$\|\Delta_{1, p_1 p_2 T}(\theta_a, \theta_b)\|_{\psi_2} \lesssim d(\theta_a, \theta_b) \quad \text{and} \quad \|\Delta_{2, p_1 p_2 T}(\theta_a, \theta_b)\|_{\psi_2} \lesssim d(\theta_a, \theta_b).$$

Thus,

$$\|\Delta_{p_1 p_2 T}(\theta_a, \theta_b)\|_{\psi_2} \lesssim \|\Delta_{1, p_1 p_2 T}(\theta_a, \theta_b)\|_{\psi_2} + \|\Delta_{2, p_1 p_2 T}(\theta_a, \theta_b)\|_{\psi_2} \lesssim d(\theta_a, \theta_b).$$

Therefore, similar to the proof of Lemma F.3, we can show that for sufficiently small  $\delta > 0$ ,

$$\mathbb{E} \left[ \sup_{\theta \in \Theta^{k_1 k_2}(\delta)} |\mathbb{V}_{p_1 p_2 T}(\theta)| \right] \lesssim \frac{\delta}{L_{p_1 p_2 T} h}. \quad (64)$$

It then follows from (64) and Lemma F.3 that  $\mathbb{V}_{p_1 p_2 T}(\tilde{\theta}) = O_p(1/(L_{p_1 p_2 T}^2 h)) = O_p(1/(T p_2 h))$ , for example, the fifth term on the right of (63) is  $O_p(1/(T p_2 h))$ . Similar results can be obtained for the fourth and sixth terms on the right of (63), and thus the desired result follows.  $\square$

**Lemma F.8.** *Under Assumptions 1 and 2, for each  $i$  and  $j$  we have*

$$\frac{1}{T} \sum_{t=1}^T \tilde{\rho}_{ijt}^{(1)}(\tilde{F}_t - F_{0t}) = O_p\left(\frac{1}{T p_2 h}\right), \quad \frac{1}{T} \sum_{t=1}^T \tilde{\rho}_{ijt}^{(2)} F_{0t}(\tilde{F}_t - F_{0t})' = O_p\left(\frac{1}{T p_2 h^2}\right),$$

for each  $i$  and  $t$  we have

$$\frac{1}{p_2} \sum_{j=1}^{p_2} \tilde{\rho}_{ijt}^{(1)} (\tilde{c}_j - c_{0j}) = O_p\left(\frac{1}{Tp_2h}\right), \quad \frac{1}{p_2} \sum_{j=1}^{p_2} \tilde{\rho}_{ijt}^{(2)} c_{0j} (\tilde{c}_j - c_{0j})' = O_p\left(\frac{1}{Tp_2h^2}\right).$$

*Proof.* To save space, we only prove the second result of  $\tilde{F}_t$ , since the proof of the first result is similar. Using (58) and (62), we can write

$$\begin{aligned} & \frac{1}{T} \sum_{t=1}^T \tilde{\rho}_{ijt}^{(2)} F_{0t} (\tilde{F}_t - F_{0t})' \\ &= \frac{1}{Tp_1p_2} \sum_{l=1}^{p_1} \sum_{t=1}^T \sum_{k=1}^{p_2} \tilde{\rho}_{ijt}^{(2)} \tilde{\rho}_{ltk}^{(1)} F_{0t} c_{0k} r'_{0l} (\Psi_{p_1p_2,t})^{-1} \\ &+ \frac{1}{p_1p_2T} \sum_{l=1}^{p_1} \sum_{t=1}^T \sum_{k=1}^{p_2} \tilde{\rho}_{ijt}^{(2)} F_{0t} \{ \tilde{\rho}^{(1)}(X_{ltk} - \tilde{r}'_l \tilde{F}_t \tilde{c}_k) \tilde{c}_k \tilde{r}'_l - \tilde{\rho}_{ltk}^{(1)} c_{0k} r'_{0l} (\Psi_{p_1p_2,t})^{-1} \} \\ &- \frac{1}{\sqrt{p_1p_2T}} \sum_{l=1}^{p_1} \sum_{s=1}^T \sum_{k=1}^{p_2} \left( \frac{1}{T} \sum_{t=1}^T \tilde{\rho}_{ijt}^{(2)} F_{0t} \tilde{c}_k \tilde{F}'_s \mathcal{D}_{t,l}^{FR'} \right) \tilde{\rho}^{(1)}(X_{lsk} - \tilde{r}'_l \tilde{F}_s \tilde{c}_k) \\ &- \frac{1}{\sqrt{p_1p_2T}} \sum_{l=1}^{p_1} \sum_{s=1}^T \sum_{k=1}^{p_2} \left( \frac{1}{T} \sum_{t=1}^T \tilde{\rho}_{ijt}^{(2)} F_{0t} \tilde{c}_k \tilde{r}'_l \mathcal{D}_{t,s}^{FF'} \right) \tilde{\rho}^{(1)}(X_{lsk} - \tilde{r}'_l \tilde{F}_s \tilde{c}_k) \\ &- \frac{1}{\sqrt{p_1p_2T}} \sum_{l=1}^{p_1} \sum_{s=1}^T \sum_{k=1}^{p_2} \left( \frac{1}{T} \sum_{t=1}^T \tilde{\rho}_{ijt}^{(2)} F_{0t} \tilde{r}'_l \tilde{F}_s \mathcal{D}_{t,k}^{FC'} \right) \tilde{\rho}^{(1)}(X_{lsk} - \tilde{r}'_l \tilde{F}_s \tilde{c}_k) \\ &+ \frac{1}{2T} \sum_{t=1}^T \tilde{\rho}_{ijt}^{(2)} F_{0t} \mathcal{R}'(\tilde{\theta})_{p_1+t} (\Psi_{p_1p_2,t})^{-1} + \frac{1}{2T} \sum_{t=1}^T \sum_{l=1}^{p_1} \tilde{\rho}_{ijt}^{(2)} F_{0t} \mathcal{R}'(\tilde{\theta})_l \mathcal{D}_{t,l}^{FR'} \\ &+ \frac{1}{2T} \sum_{t=1}^T \tilde{\rho}_{ijt}^{(2)} F_{0t} \mathcal{R}'(\tilde{\theta})_{p_1+s} \mathcal{D}_{t,s}^{FF'} + \frac{1}{2T} \sum_{t=1}^T \tilde{\rho}_{ijt}^{(2)} F_{0t} \mathcal{R}'(\tilde{\theta})_{p_1+T+k} \mathcal{D}_{t,k}^{FC'} + \bar{O}(h^m). \end{aligned} \quad (65)$$

First, we can write

$$\begin{aligned} & \frac{1}{Tp_1p_2} \sum_{l=1}^{p_1} \sum_{t=1}^T \sum_{k=1}^{p_2} \tilde{\rho}_{ijt}^{(2)} \tilde{\rho}_{ltk}^{(1)} F_{0t} c_{0k} r'_{0l} (\Psi_{p_1p_2,t})^{-1} \\ &= \frac{1}{Tp_1p_2} \sum_{t=1}^T \tilde{\rho}_{ijt}^{(2)} \tilde{\rho}_{ijt}^{(1)} F_{0t} c_{0j} r'_{0i} (\Psi_{p_1p_2,t})^{-1} + \frac{1}{Tp_1p_2} \sum_{t=1}^T \sum_{l=1, l \neq i}^{p_1} \sum_{k=1, k \neq j}^{p_2} \tilde{\rho}_{ijt}^{(2)} \tilde{\rho}_{ltk}^{(1)} F_{0t} c_{0k} r'_{0l} (\Psi_{p_1p_2,t})^{-1}. \end{aligned}$$

Since  $h\tilde{\rho}_{ijt}^{(2)}(\cdot)$  is uniformly bounded by Lemma F.1,  $\max_{t \leq T} \|(\Psi_{p_1p_2,t})^{-1}\| = O(1)$  for large  $p_1, p_2$  by Assumption 2, the first term on the RHS of the above equation is  $O_p((p_1p_2h)^{-1})$ . Using Lyapunov's CLT and Lemma F.1, the second term on the RHS of the above equation can be shown to be  $O_p((Tp_1p_2h)^{-\frac{1}{2}})$ . Thus, the first term on the RHS of (65) is  $O_p(Tp_2h)^{-1}$ .

Second, consider the second term on the RHS of (65), which can be written as

$$O_p\left(\frac{1}{p_1 p_2 h}\right) + \frac{1}{T p_1 p_2} \sum_{t=1}^T \sum_{l=1, l \neq i}^{p_1} \sum_{k=1, k \neq j}^{p_2} \tilde{\rho}_{ijt}^{(2)} F_{0t} \{\tilde{\rho}^{(1)}(X_{ltk} - \tilde{r}_l' \tilde{F}_t \tilde{c}_k) \tilde{c}_k \tilde{r}_l' - \tilde{\rho}_{ltk}^{(1)} c_{0k} r_{0l}' (\Psi_{p_1 p_2, t})^{-1}\}.$$

Similar to the proof of Lemma F.7, the second term of the above expression can be shown to be  $O_p(1/(T p_2 h^2))$ . So the second term on the RHS of (65) is  $O_p(1/(T p_2 h^2))$ .

Next, for the third term on the RHS of (65), its  $p, q$ th element is given by

$$\frac{1}{\sqrt{p_1 p_2 T}} \sum_{l=1}^{p_1} \sum_{s=1}^T \sum_{k=1}^{p_2} \mathcal{X}_{i,j,l} \bar{\rho}^{(1)}(X_{lsk} - \tilde{r}_l' \tilde{F}_s \tilde{c}_k),$$

where  $\mathcal{X}_{i,j,l} = \frac{1}{T} \sum_{t=1}^T (\sqrt{p_1 p_2 T} \mathcal{D}_{t,l,q}^{FR}) F_{0t,p} \tilde{\rho}_{ijt}^{(2)}$ , and  $F_{0t,p}$  is the  $p$ th row of  $F_{0t}$ ,  $\mathcal{D}_{t,l,q}^{FR}$  is the  $q$ th ‘column’ of  $\mathcal{D}_{t,l}^{FR}$ . Therefore,

$$\begin{aligned} & \left\| \frac{1}{\sqrt{p_1 p_2 T}} \sum_{l=1}^{p_1} \sum_{s=1}^T \sum_{k=1}^{p_2} \mathcal{X}_{i,j,l} \bar{\rho}^{(1)}(X_{lsk} - \tilde{r}_l' \tilde{F}_s \tilde{c}_k) \right\| \\ & \leq \sqrt{\frac{1}{p_1} \sum_{l=1}^{p_1} \|\mathcal{X}_{i,j,l}\|^2} \cdot \sqrt{\frac{1}{p_1 p_2 T} \sum_{l=1}^{p_1} \sum_{s=1}^T \sum_{k=1}^{p_2} [\bar{\rho}^{(1)}(X_{lsk} - \tilde{r}_l' \tilde{F}_s \tilde{c}_k)]^2 \|\tilde{F}_s \tilde{c}_k\|^2}. \end{aligned}$$

Since  $|\sqrt{p_1 p_2 T} F_{0t} \mathcal{D}_{t,l}^{FR}|$  is uniformly bounded by Lemma F.6, it can be shown that  $\mathbb{E}\|\mathcal{X}_{i,j,l}\|^2 = O((T p_2 h)^{-1})$ . Moreover,

$$\begin{aligned} [\bar{\rho}^{(1)}(X_{lsk} - \tilde{r}_l' \tilde{F}_s \tilde{c}_k)]^2 &= [\bar{\rho}_{ijt}^{(1)} + \bar{\rho}^{(2)}(X_{lsk} - r_l^{*'} F_s^* c_k^*) \cdot (r_{0i}' F_{0t} c_{0j} - \tilde{r}_l' \tilde{F}_s \tilde{c}_k)]^2 \\ &\leq O(h^{2m}) + (r_{0i}' F_{0t} c_{0j} - \tilde{r}_l' \tilde{F}_s \tilde{c}_k)^2, \end{aligned}$$

thus,

$$\sqrt{\frac{1}{p_1 p_2 T} \sum_{l=1}^{p_1} \sum_{s=1}^T \sum_{k=1}^{p_2} [\bar{\rho}^{(1)}(X_{lsk} - \tilde{r}_l' \tilde{F}_s \tilde{c}_k)]^2 \|\tilde{F}_s \tilde{c}_k\|^2} \leq O(h^{2m}) + d(\tilde{\theta}, \theta_0) = O_p(1/L_{p_1 p_2 T})$$

by Lemma F.3. So, the third term on the RHS of (65) is  $O_p((T p_2)^{-1} h^{-\frac{1}{2}})$ , while the fourth term on the RHS of (65) can be shown to be  $O_p((T p_2)^{-1} h^{-\frac{1}{2}})$  in the same way.

Finally, it follows from Lemma F.3 and (60) that the sixth term on the RHS of (65) is  $O_p((L_{p_1 p_2 T})^{-2} h^{-1}) = O_p((T p_2 h)^{-1})$ . The  $p, q$ th element of the seventh term on the RHS of (65)

can be written as  $(2\sqrt{p_1 p_2 T})^{-1} \sum_{l=1}^{p_1} \mathcal{X}_{i,j,l} \mathcal{R}(\tilde{\theta})_l$ , which is bounded by

$$\frac{\sqrt{p_1}}{2\sqrt{p_2 T}} \sqrt{\frac{1}{p_1} \sum_{l=1}^{p_1} \|\mathcal{X}_{i,j,l}\|^2} \sqrt{\frac{1}{p_1} \sum_{l=1}^{p_1} \|\mathcal{R}(\tilde{\theta})_l\|^2} = O_p((Tp_2 h)^{-\frac{1}{2}}) O_p((L_{p_1 p_2 T})^{-2}) = O_p((Tp_2)^{-\frac{3}{2}} h^{-\frac{1}{2}}).$$

The same bound for the seventh term on the RHS of (65) can be obtained using the same argument.

Thus, combining the above results, we get

$$\frac{1}{T} \sum_{t=1}^T \tilde{\rho}_{ijt}^{(2)} F_{0t} (\tilde{F}_t - F_{0t})' = O_p\left(\frac{1}{Tp_2 h^2}\right).$$

□

## F.2 Proof of Theorem 5.1

*Proof.* From the expansion in the proof of Lemma F.5, we have

$$\begin{aligned} (**) \Phi_{Tp_2, i}(\tilde{r}_i - r_{0i}) &= -\frac{1}{Tp_2} \sum_{t=1}^T \sum_{j=1}^{p_2} \bar{\rho}^{(1)}(X_{ijt} - \tilde{r}_i' \tilde{F}_t \tilde{c}_j) \tilde{F}_t \tilde{c}_j + \frac{1}{Tp_2} \sum_{t=1}^T \sum_{j=1}^{p_2} \bar{\rho}_{ijt}^{(1)} F_{0t} c_{0j} \\ &\quad + \frac{1}{Tp_2} \sum_{t=1}^T \sum_{j=1}^{p_2} \bar{\rho}_{ijt}^{(1)} (\tilde{F}_t - F_{0t}) \tilde{c}_j + \frac{1}{Tp_2} \sum_{t=1}^T \sum_{j=1}^{p_2} \bar{\rho}_{ijt}^{(1)} F_{0t} (\tilde{c}_j - c_{0j}) \\ &\quad - \frac{1}{Tp_2} \sum_{t=1}^T \sum_{j=1}^{p_2} \bar{\rho}_{ijt}^{(2)} F_{0t} c_{0j} r'_{0i} (\tilde{F}_t - F_{0t})' \tilde{c}_j - \frac{1}{Tp_2} \sum_{t=1}^T \sum_{j=1}^{p_2} \bar{\rho}_{ijt}^{(2)} F_{0t} c_{0j} r'_{0i} F_{0t} (\tilde{c}_j - c_{0j}) \\ &\quad + \frac{1}{Tp_2} \sum_{t=1}^T \sum_{j=1}^{p_2} \bar{\rho}_{ijt}^{(3)} \tilde{F}_t \tilde{c}_j \tilde{c}_j' \tilde{F}_t' (\tilde{r}_i - r_{0i}) r'_{0i} (\tilde{F}_t - F_{0t}) \tilde{c}_j \\ &\quad + \frac{1}{Tp_2} \sum_{t=1}^T \sum_{j=1}^{p_2} \bar{\rho}_{ijt}^{(3)} \tilde{F}_t \tilde{c}_j \tilde{c}_j' \tilde{F}_t' (\tilde{r}_i - r_{0i}) r'_{0i} F_{0t} (\tilde{c}_j - c_{0j}) + o_p(\|\tilde{r}_i - r_{0i}\|). \end{aligned}$$

Then, it follows from Lemmas F.1, F.3 and F.7 that

$$\Phi_{Tp_2, i}(\tilde{r}_i - r_{0i}) = -\frac{1}{Tp_2} \sum_{t=1}^T \sum_{j=1}^{p_2} \bar{\rho}^{(1)}(X_{ijt} - \tilde{r}_i' \tilde{F}_t \tilde{c}_j) \tilde{F}_t \tilde{c}_j + O(h^m) + O_p\left(\frac{1}{Tp_2 h}\right) + o_p(\|\tilde{r}_i - r_{0i}\|).$$

Note that

$$\begin{aligned}
& -\frac{1}{Tp_2} \sum_{t=1}^T \sum_{j=1}^{p_2} \bar{\rho}^{(1)}(X_{ijt} - \tilde{r}'_i \tilde{F}_t \tilde{c}_j) \tilde{F}_t \tilde{c}_j \\
& = \frac{1}{Tp_2} \sum_{t=1}^T \sum_{j=1}^{p_2} \tilde{\rho}^{(1)}(X_{ijt} - \tilde{r}'_i \tilde{F}_t \tilde{c}_j) \tilde{F}_t \tilde{c}_j \\
& = \frac{1}{Tp_2} \sum_{t=1}^T \sum_{j=1}^{p_2} \tilde{\rho}_{ijt}^{(1)} \tilde{F}_t \tilde{c}_j - \frac{1}{Tp_2} \sum_{t=1}^T \sum_{j=1}^{p_2} \tilde{\rho}_{ijt}^{(2)} (\tilde{r}'_i \tilde{F}_t \tilde{c}_j - r'_{0i} F_{0t} c_{0j}) \tilde{F}_t \tilde{c}_j \\
& \quad + 0.5 \frac{1}{Tp_2} \sum_{t=1}^T \sum_{j=1}^{p_2} \tilde{\rho}_{ijt}^{(3)} (*) (\tilde{r}'_i \tilde{F}_t \tilde{c}_j - r'_{0i} F_{0t} c_{0j})^2 \tilde{F}_t \tilde{c}_j,
\end{aligned}$$

where  $\tilde{\rho}_{ijt}^{(3)}(*) = \tilde{\rho}_{ijt}^{(3)}(c_{ijt}^*)$  and  $c_{ijt}^*$  is between  $r'_{0i} F_{0t} c_{0j}$  and  $\tilde{r}'_i \tilde{F}_t \tilde{c}_j$ .

First, by Lemma F.8 (i), we have

$$\begin{aligned}
& \frac{1}{Tp_2} \sum_{t=1}^T \sum_{j=1}^{p_2} \tilde{\rho}_{ijt}^{(1)} \tilde{F}_t \tilde{c}_j \\
& = \frac{1}{Tp_2} \sum_{t=1}^T \sum_{j=1}^{p_2} \tilde{\rho}_{ijt}^{(1)} F_{0t} c_{0j} + \frac{1}{Tp_2} \sum_{t=1}^T \sum_{j=1}^{p_2} \tilde{\rho}_{ijt}^{(1)} (\tilde{F}_t \tilde{c}_j - F_{0t} c_{0j}) \\
& = \frac{1}{Tp_2} \sum_{t=1}^T \sum_{j=1}^{p_2} \tilde{\rho}_{ijt}^{(1)} F_{0t} c_{0j} + \frac{1}{Tp_2} \sum_{t=1}^T \sum_{j=1}^{p_2} \tilde{\rho}_{ijt}^{(1)} (\tilde{F}_t - F_{0t}) \tilde{c}_j + \frac{1}{Tp_2} \sum_{t=1}^T \sum_{j=1}^{p_2} \tilde{\rho}_{ijt}^{(1)} F_{0t} (\tilde{c}_j - c_{0j}) \\
& = \frac{1}{Tp_2} \sum_{t=1}^T \sum_{j=1}^{p_2} \tilde{\rho}_{ijt}^{(1)} F_{0t} c_{0j} + O_p\left(\frac{1}{Tp_2 h}\right).
\end{aligned}$$

Second,

$$\begin{aligned}
& \frac{1}{Tp_2} \sum_{t=1}^T \sum_{j=1}^{p_2} \tilde{\rho}_{ijt}^{(2)} (\tilde{r}'_i \tilde{F}_t \tilde{c}_j - r'_{0i} F_{0t} c_{0j}) \tilde{F}_t \tilde{c}_j \\
& = \frac{1}{Tp_2} \sum_{t=1}^T \sum_{j=1}^{p_2} \tilde{\rho}_{ijt}^{(2)} \tilde{F}_t \tilde{c}_j c'_{0j} F'_{0t} (\tilde{r}_i - r_{0i}) + \frac{1}{Tp_2} \sum_{t=1}^T \sum_{j=1}^{p_2} \tilde{\rho}_{ijt}^{(2)} \tilde{F}_t \tilde{c}_j c'_{0j} (\tilde{F}_t - F_{0t})' \tilde{r}_i \\
& \quad + \frac{1}{Tp_2} \sum_{t=1}^T \sum_{j=1}^{p_2} \tilde{\rho}_{ijt}^{(2)} \tilde{F}_t \tilde{c}_j (\tilde{c}_j - c_{0j})' \tilde{F}_t' \tilde{r}_i \\
& = (1) + (2) + (3).
\end{aligned}$$

Note that

$$\begin{aligned}
(1) &= \frac{1}{Tp_2} \sum_{t=1}^T \sum_{j=1}^{p_2} \tilde{\rho}_{ijt}^{(2)} \tilde{F}_t \tilde{c}_j c'_{0j} F'_{0t} (\tilde{r}_i - r_{0i}) \\
&= \frac{1}{Tp_2} \sum_{t=1}^T \sum_{j=1}^{p_2} \tilde{\rho}_{ijt}^{(2)} F_{0t} c_{0j} c'_{0j} F'_{0t} (\tilde{r}_i - r_{0i}) + \frac{1}{Tp_2} \sum_{t=1}^T \sum_{j=1}^{p_2} \tilde{\rho}_{ijt}^{(2)} (\tilde{F}_t \tilde{c}_j - F_{0t} c_{0j}) c'_{0j} F'_{0t} (\tilde{r}_i - r_{0i}) \\
&= \frac{1}{Tp_2} \sum_{t=1}^T \sum_{j=1}^{p_2} \tilde{\rho}_{ijt}^{(2)} F_{0t} c_{0j} c'_{0j} F'_{0t} (\tilde{r}_i - r_{0i}) + \frac{1}{Tp_2} \sum_{t=1}^T \sum_{j=1}^{p_2} \tilde{\rho}_{ijt}^{(2)} (\tilde{F}_t - F_{0t}) \tilde{c}_j c'_{0j} F'_{0t} (\tilde{r}_i - r_{0i}) \\
&\quad + \frac{1}{Tp_2} \sum_{t=1}^T \sum_{j=1}^{p_2} \tilde{\rho}_{ijt}^{(2)} F_{0t} (\tilde{c}_j - c_{0j}) c'_{0j} F'_{0t} (\tilde{r}_i - r_{0i}).
\end{aligned}$$

It follows from Lemma F.1 and Lemma F.8 (ii) that (1) is  $o_p(\|\tilde{r}_i - r_{0i}\|)$ .

Note that

$$\begin{aligned}
(2) &= \frac{1}{Tp_2} \sum_{t=1}^T \sum_{j=1}^{p_2} \tilde{\rho}_{ijt}^{(2)} \tilde{F}_t \tilde{c}_j c'_{0j} (\tilde{F}_t - F_{0t})' \tilde{r}_i \\
&= \frac{1}{Tp_2} \sum_{t=1}^T \sum_{j=1}^{p_2} \tilde{\rho}_{ijt}^{(2)} F_{0t} \tilde{c}_j c'_{0j} (\tilde{F}_t - F_{0t})' \tilde{r}_i + \frac{1}{Tp_2} \sum_{t=1}^T \sum_{j=1}^{p_2} \tilde{\rho}_{ijt}^{(2)} (\tilde{F}_t - F_{0t}) \tilde{c}_j c'_{0j} (\tilde{F}_t - F_{0t})' \tilde{r}_i.
\end{aligned}$$

Lemma F.8 (ii) implies that the first term of (2) is  $O_p(1/Tp_2h^2)$  and Lemma F.3 implies that the second term of (2) is  $O_p(1/Tp_2h)$ .

Note that

$$\begin{aligned}
(3) &= \frac{1}{Tp_2} \sum_{t=1}^T \sum_{j=1}^{p_2} \tilde{\rho}_{ijt}^{(2)} \tilde{F}_t \tilde{c}_j (\tilde{c}_j - c_{0j})' \tilde{F}_t' \tilde{r}_i \\
&= \frac{1}{Tp_2} \sum_{t=1}^T \sum_{j=1}^{p_2} \tilde{\rho}_{ijt}^{(2)} \tilde{F}_t c_{0j} (\tilde{c}_j - c_{0j})' \tilde{F}_t' \tilde{r}_i + \frac{1}{Tp_2} \sum_{t=1}^T \sum_{j=1}^{p_2} \tilde{\rho}_{ijt}^{(2)} \tilde{F}_t (\tilde{c}_j - c_{0j}) (\tilde{c}_j - c_{0j})' \tilde{F}_t' \tilde{r}_i \\
&= \frac{1}{Tp_2} \sum_{t=1}^T \sum_{j=1}^{p_2} \tilde{\rho}_{ijt}^{(2)} F_{0t} c_{0j} (\tilde{c}_j - c_{0j})' \tilde{F}_t' \tilde{r}_i + \frac{1}{Tp_2} \sum_{t=1}^T \sum_{j=1}^{p_2} \tilde{\rho}_{ijt}^{(2)} (\tilde{F}_t - F_{0t}) c_{0j} (\tilde{c}_j - c_{0j})' \tilde{F}_t' \tilde{r}_i \\
&\quad + \frac{1}{Tp_2} \sum_{t=1}^T \sum_{j=1}^{p_2} \tilde{\rho}_{ijt}^{(2)} \tilde{F}_t (\tilde{c}_j - c_{0j}) (\tilde{c}_j - c_{0j})' \tilde{F}_t' \tilde{r}_i \\
&= \frac{1}{Tp_2} \sum_{t=1}^T \sum_{j=1}^{p_2} \tilde{\rho}_{ijt}^{(2)} F_{0t} c_{0j} (\tilde{c}_j - c_{0j})' F_{0t}' \tilde{r}_i + \frac{1}{Tp_2} \sum_{t=1}^T \sum_{j=1}^{p_2} \tilde{\rho}_{ijt}^{(2)} F_{0t} c_{0j} (\tilde{c}_j - c_{0j})' (\tilde{F}_t - F_{0t})' \tilde{r}_i \\
&\quad + \frac{1}{Tp_2} \sum_{t=1}^T \sum_{j=1}^{p_2} \tilde{\rho}_{ijt}^{(2)} (\tilde{F}_t - F_{0t}) c_{0j} (\tilde{c}_j - c_{0j})' \tilde{F}_t' \tilde{r}_i + \frac{1}{Tp_2} \sum_{t=1}^T \sum_{j=1}^{p_2} \tilde{\rho}_{ijt}^{(2)} \tilde{F}_t (\tilde{c}_j - c_{0j}) (\tilde{c}_j - c_{0j})' \tilde{F}_t' \tilde{r}_i.
\end{aligned}$$

It follows from Lemma F.8 (ii) that the first three terms of (3) are  $O_p(1/Tp_2h^2)$  and Lemma F.3 implies that the last term of (3) is  $O_p(1/Tp_2h)$ .

Thus, we have

$$\frac{1}{Tp_2} \sum_{t=1}^T \sum_{j=1}^{p_2} \tilde{\rho}_{ijt}^{(2)} (\tilde{r}'_i \tilde{F}_t \tilde{c}_j - r'_{0i} F_{0t} c_{0j}) \tilde{F}_t \tilde{c}_j = O_p\left(\frac{1}{Tp_2h^2}\right) + o_p(\|\tilde{r}_i - r_{0i}\|). \quad (66)$$

Next, it is also easy to show that

$$\begin{aligned} & \left\| \frac{1}{Tp_2} \sum_{t=1}^T \sum_{j=1}^{p_2} \tilde{\rho}_{ijt}^{(3)} (*) (\tilde{r}'_i \tilde{F}_t \tilde{c}_j - r'_{0i} F_{0t} c_{0j})^2 \tilde{F}_t \tilde{c}_j \right\| \\ & \lesssim \|\tilde{r}_i - r_{0i}\|^2 \frac{1}{Tp_2} \sum_{t=1}^T \sum_{j=1}^{p_2} |\tilde{\rho}_{ijt}^{(3)} (*)| + \frac{1}{Tp_2} \sum_{t=1}^T \sum_{j=1}^{p_2} |\tilde{\rho}_{ijt}^{(3)} (*)| \|\tilde{F}_t - F_{0t}\|^2 + \frac{1}{Tp_2} \sum_{t=1}^T \sum_{j=1}^{p_2} |\tilde{\rho}_{ijt}^{(3)} (*)| \|\tilde{c}_j - c_{0j}\|^2. \end{aligned}$$

Therefore, from Lemma F.1, Lemma F.3, and Lemma F.5, we have

$$\frac{1}{Tp_2} \sum_{t=1}^T \sum_{j=1}^{p_2} \tilde{\rho}_{ijt}^{(3)} (*) (\tilde{r}'_i \tilde{F}_t \tilde{c}_j - r'_{0i} F_{0t} c_{0j})^2 \tilde{F}_t \tilde{c}_j = O_p(\|\tilde{r}_i - r_{0i}\|) \cdot O_p((Tp_2)^{-\frac{1}{2}}h^{-3}) + O_p((Tp_2)^{-1}h^{-2}),$$

which is  $o_p(\|\tilde{r}_i - r_{0i}\|) + O_p((Tp_2)^{-1}h^{-2})$  under the assumption that  $(Tp_2)^{\frac{1}{2}}h^3 \rightarrow \infty$ .

Finally, combining all the above results, we get

$$\Phi_{Tp_2,i}(\tilde{r}_i - r_{0i}) = \frac{1}{Tp_2} \sum_{t=1}^T \sum_{j=1}^{p_2} \tilde{\rho}_{ijt}^{(1)} F_{0t} c_{0j} + O_p\left(\frac{1}{Tp_2h^2}\right) + O_p(h^m) + o_p(\|\tilde{r}_i - r_{0i}\|). \quad (67)$$

From Lemma F.1, it is easy to show that

$$\begin{aligned} \Phi_{Tp_2,i} &= \frac{1}{Tp_2} \sum_{t=1}^T \sum_{j=1}^{p_2} \tilde{\rho}_{ijt}^{(2)} F_{0t} c_{0j} c'_{0j} F'_{0t} \rightarrow \Phi_i > 0, \\ \frac{1}{\sqrt{Tp_2}} \sum_{t=1}^T \sum_{j=1}^{p_2} \tilde{\rho}_{ijt}^{(1)} F_{0t} c_{0j} &\rightarrow \mathcal{N}(0, \tau(1-\tau)\Sigma_1). \end{aligned} \quad (68)$$

Since our assumption implies that  $\sqrt{Tp_2}h^2 \rightarrow \infty$  and  $\sqrt{Tp_2}h^m \rightarrow 0$ , the the desired results follow from (67) and (68).  $\square$

# References

- [1] Galvao, A. F. and K. Kato (2016). Smoothed quantile regression for panel data. *Journal of econometrics* 193(1), 92–112.
- [2] Horowitz, J. L. (1998). Bootstrap methods for median regression models. *Econometrica*, 1327–1351.
- [3] Newey, W. K. and D. McFadden (1994). Large sample estimation and hypothesis testing. *Handbook of econometrics* 4, 2111–2245.
- [4] Van Der Vaart, A. W., J. A. Wellner, A. W. van der Vaart, and J. A. Wellner (1996). *Weak convergence*. Springer.
